# Supplementary material for: Quantitative Analysis of Community Evolution in Developer Social Networks Around Open Source Software Projects
Source: arXiv:2205.09935 source file (2022-05-20)
Supplement: Supplementary file 1 [file Appendix_comparison.tex]

\section{Baseline and R\&D designs}\label{app:comparison}

%%%%%%%%%%%%%%%%%%%%%%%%%%%%%%%%%%%%%%%
\subsection*{Resolutions and Efficiency}
%%%%%%%%%%%%%%%%%%%%%%%%%%%%%%%%%%%%%%%

A thorough comparison between the non-projective ECCE simulation and the ongoing R\&D was carried out to optimize the support structure through a projective design.  
Fig.~\ref{fig:Phase-II_Momentum_res} shows a study of the obtained  momentum resolution 
%for the non-projective ECCE tracker reference design and the ongoing project R\&D on the projective mechanical structure for the ECCE tracker design 
in bins of pseudorapidity.
Similarly Fig.~\ref{fig:Phase-II_dth_res} shows the angular resolution while Fig.~\ref{fig:Phase-II_KF_eff} shows the Kalman filter efficiency as defined in Eq.~\eqref{eq:objective_KF}.

%\begin{comment}
\begin{figure*}[h!]
    \centering
    \includegraphics[width=0.98\textwidth]{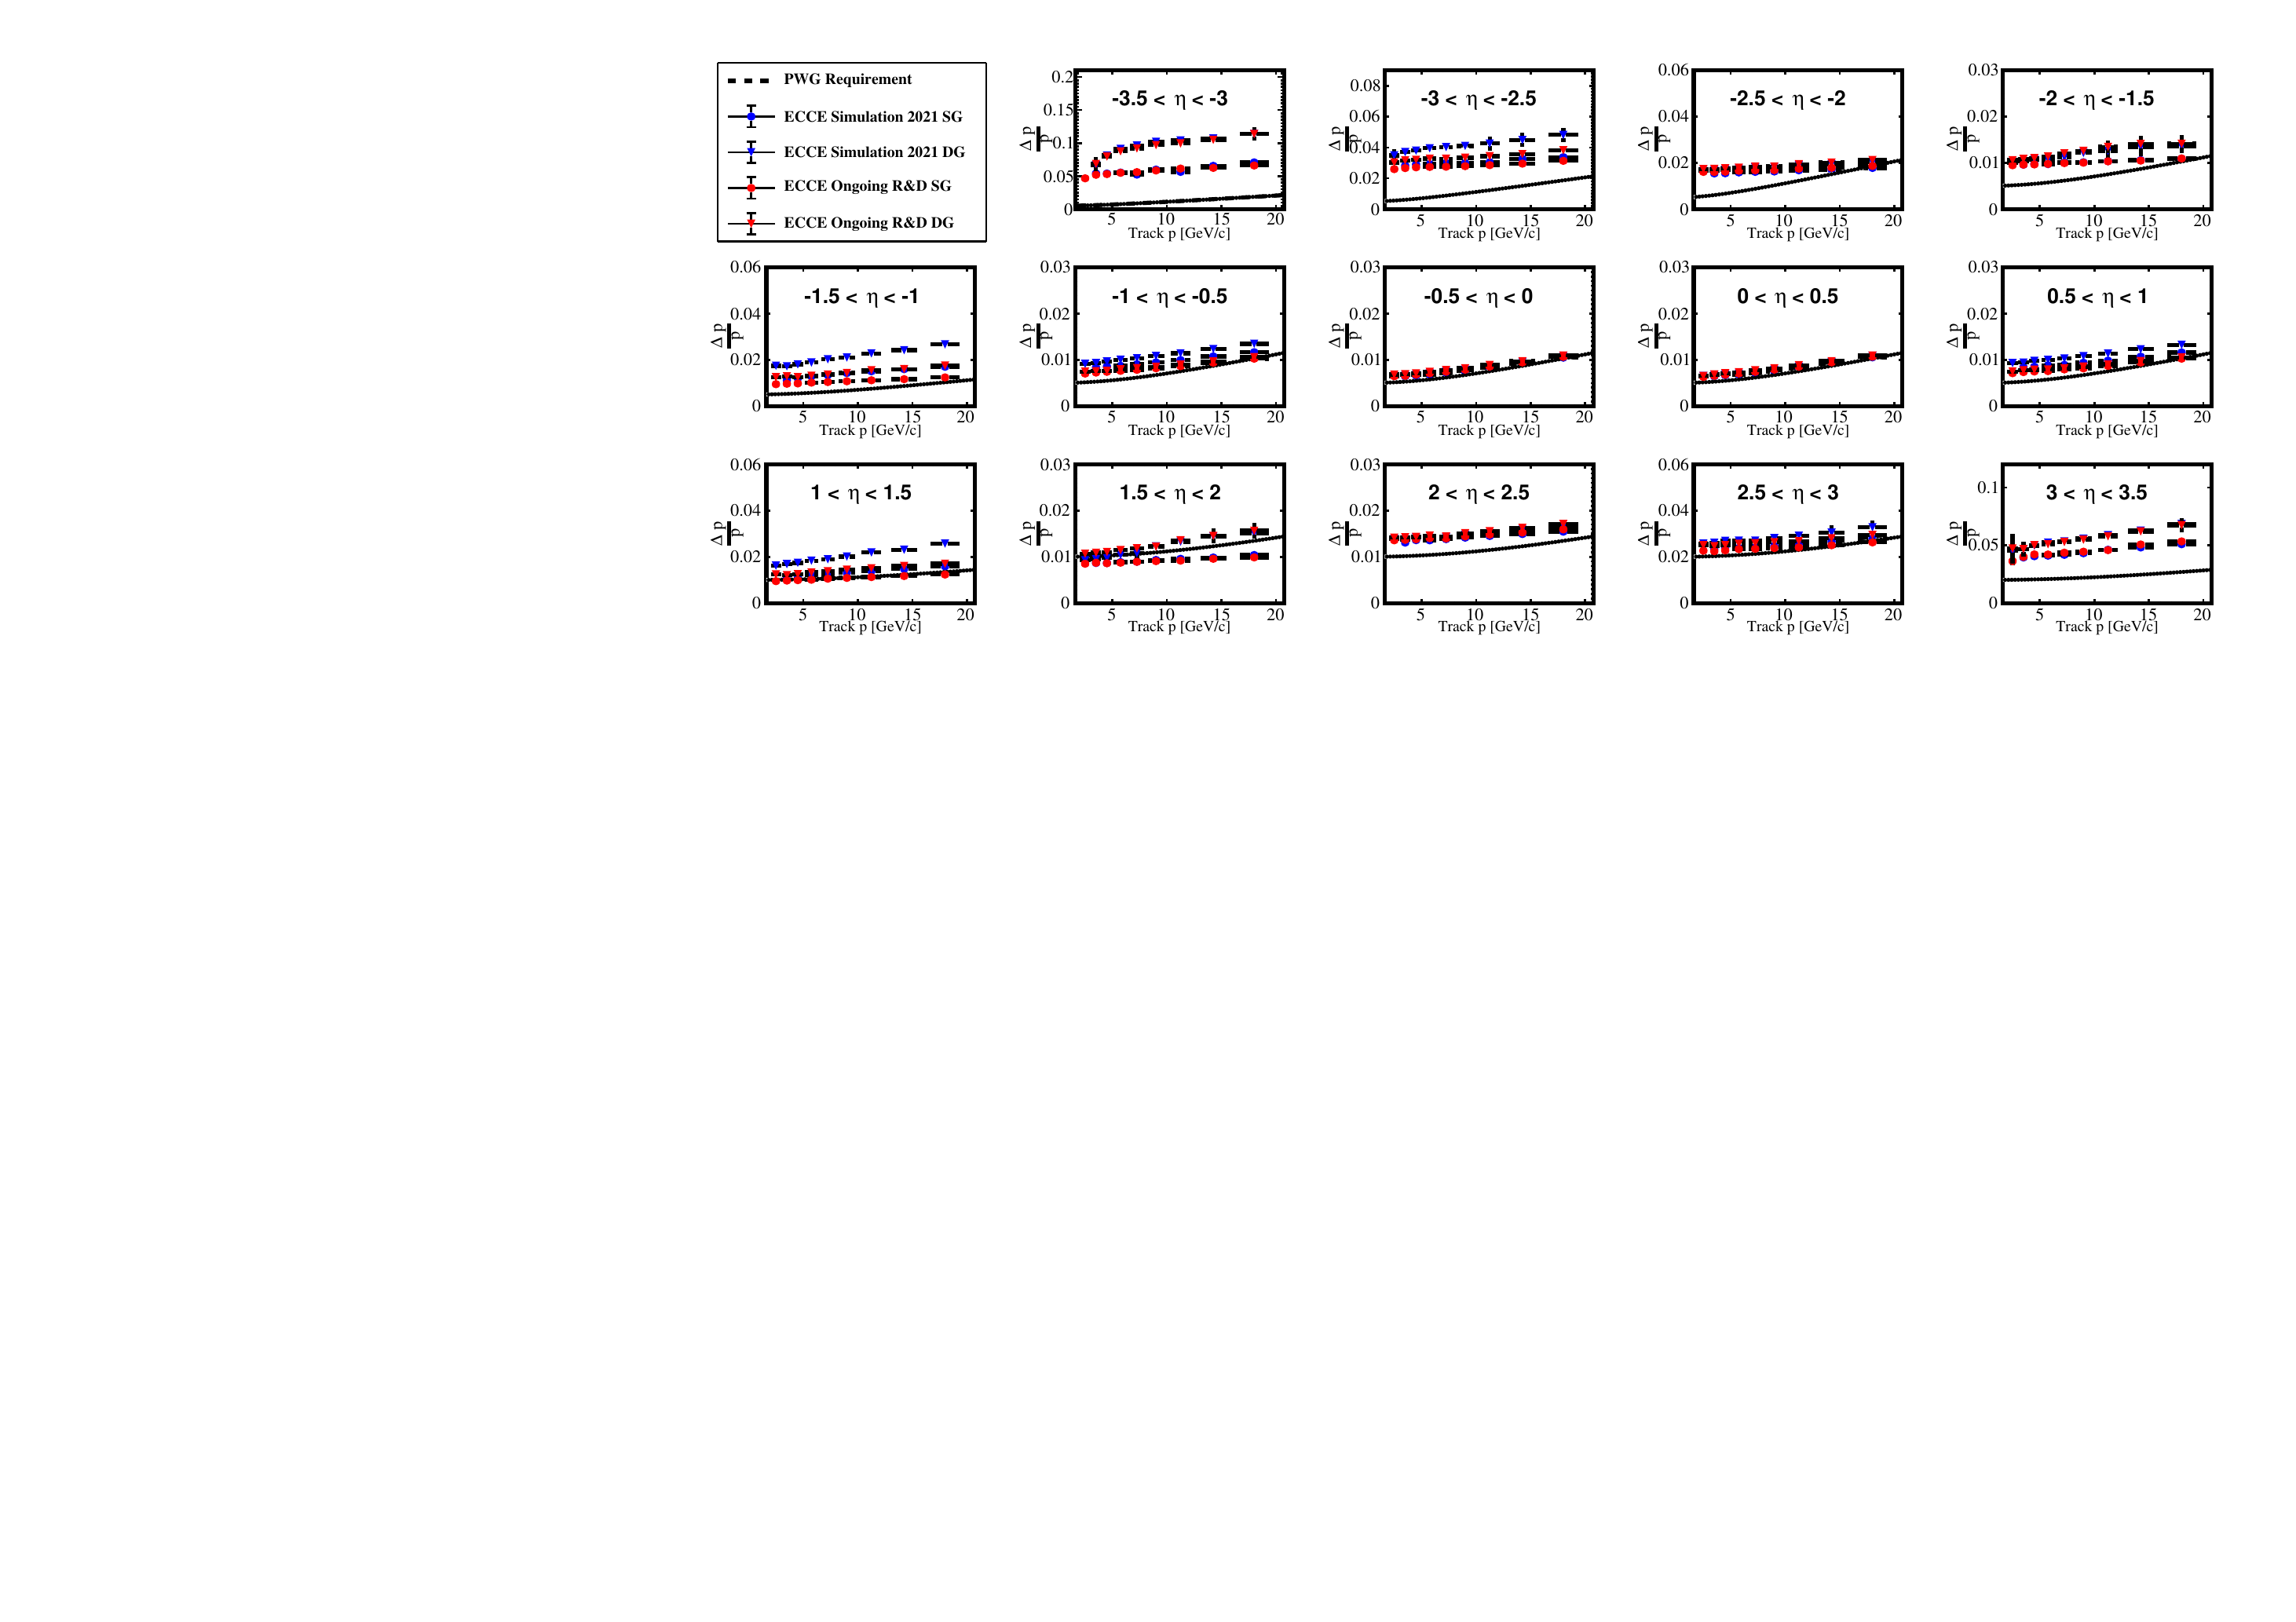}
    \caption{
    \textbf{Momentum resolution for the ECCE tracker reference design and the projective design (ongoing R\&D):} The $\Delta p /p$ are extracted with single-gaussian (SG) fits (circles) to be consistent with the YR PWG and compared to double-gaussian (DG) fits (triangles). DG (see Eq.~\eqref{eq:DG}) is used in the AI-assisted pipelines as it provides more stable fits. DG results are systematically larger than the SG ones as they capture more realistic distributions (see Fig.~\ref{fig:double_gauss}). 
    This effect is larger in $1<|\eta|<1.5$ for the non-projective design (blue points) since more material is traversed by the tracks; the same effect is moderately present also in $0.5<|\eta|<1$ for the same reason. 
    In the same bins, the ongoing R\&D design shows a significant reduction of the impact of the readout and services and SG (red circle) and DG (red triangles) are close to each other.  
    DG points are systematically large in $3<\eta<3.5$ and in $-3.5<\eta<3.0$, and this corresponds to edge effects at large $|\eta|$ values close to the inner radii of the disks in the endcaps.  
    In the region $-1<\eta<3.0$ $\Delta p/p$ is consistent with the YR physics requirements with SG. Note that physics in the backward region relies on the EM calorimeter also, and in the proposal it has been demonstrated that larger resolutions are acceptable.  
    \label{fig:Phase-II_Momentum_res}
    }
\end{figure*}

\begin{figure*}[!]
    \centering
    \includegraphics[width=0.98\textwidth]{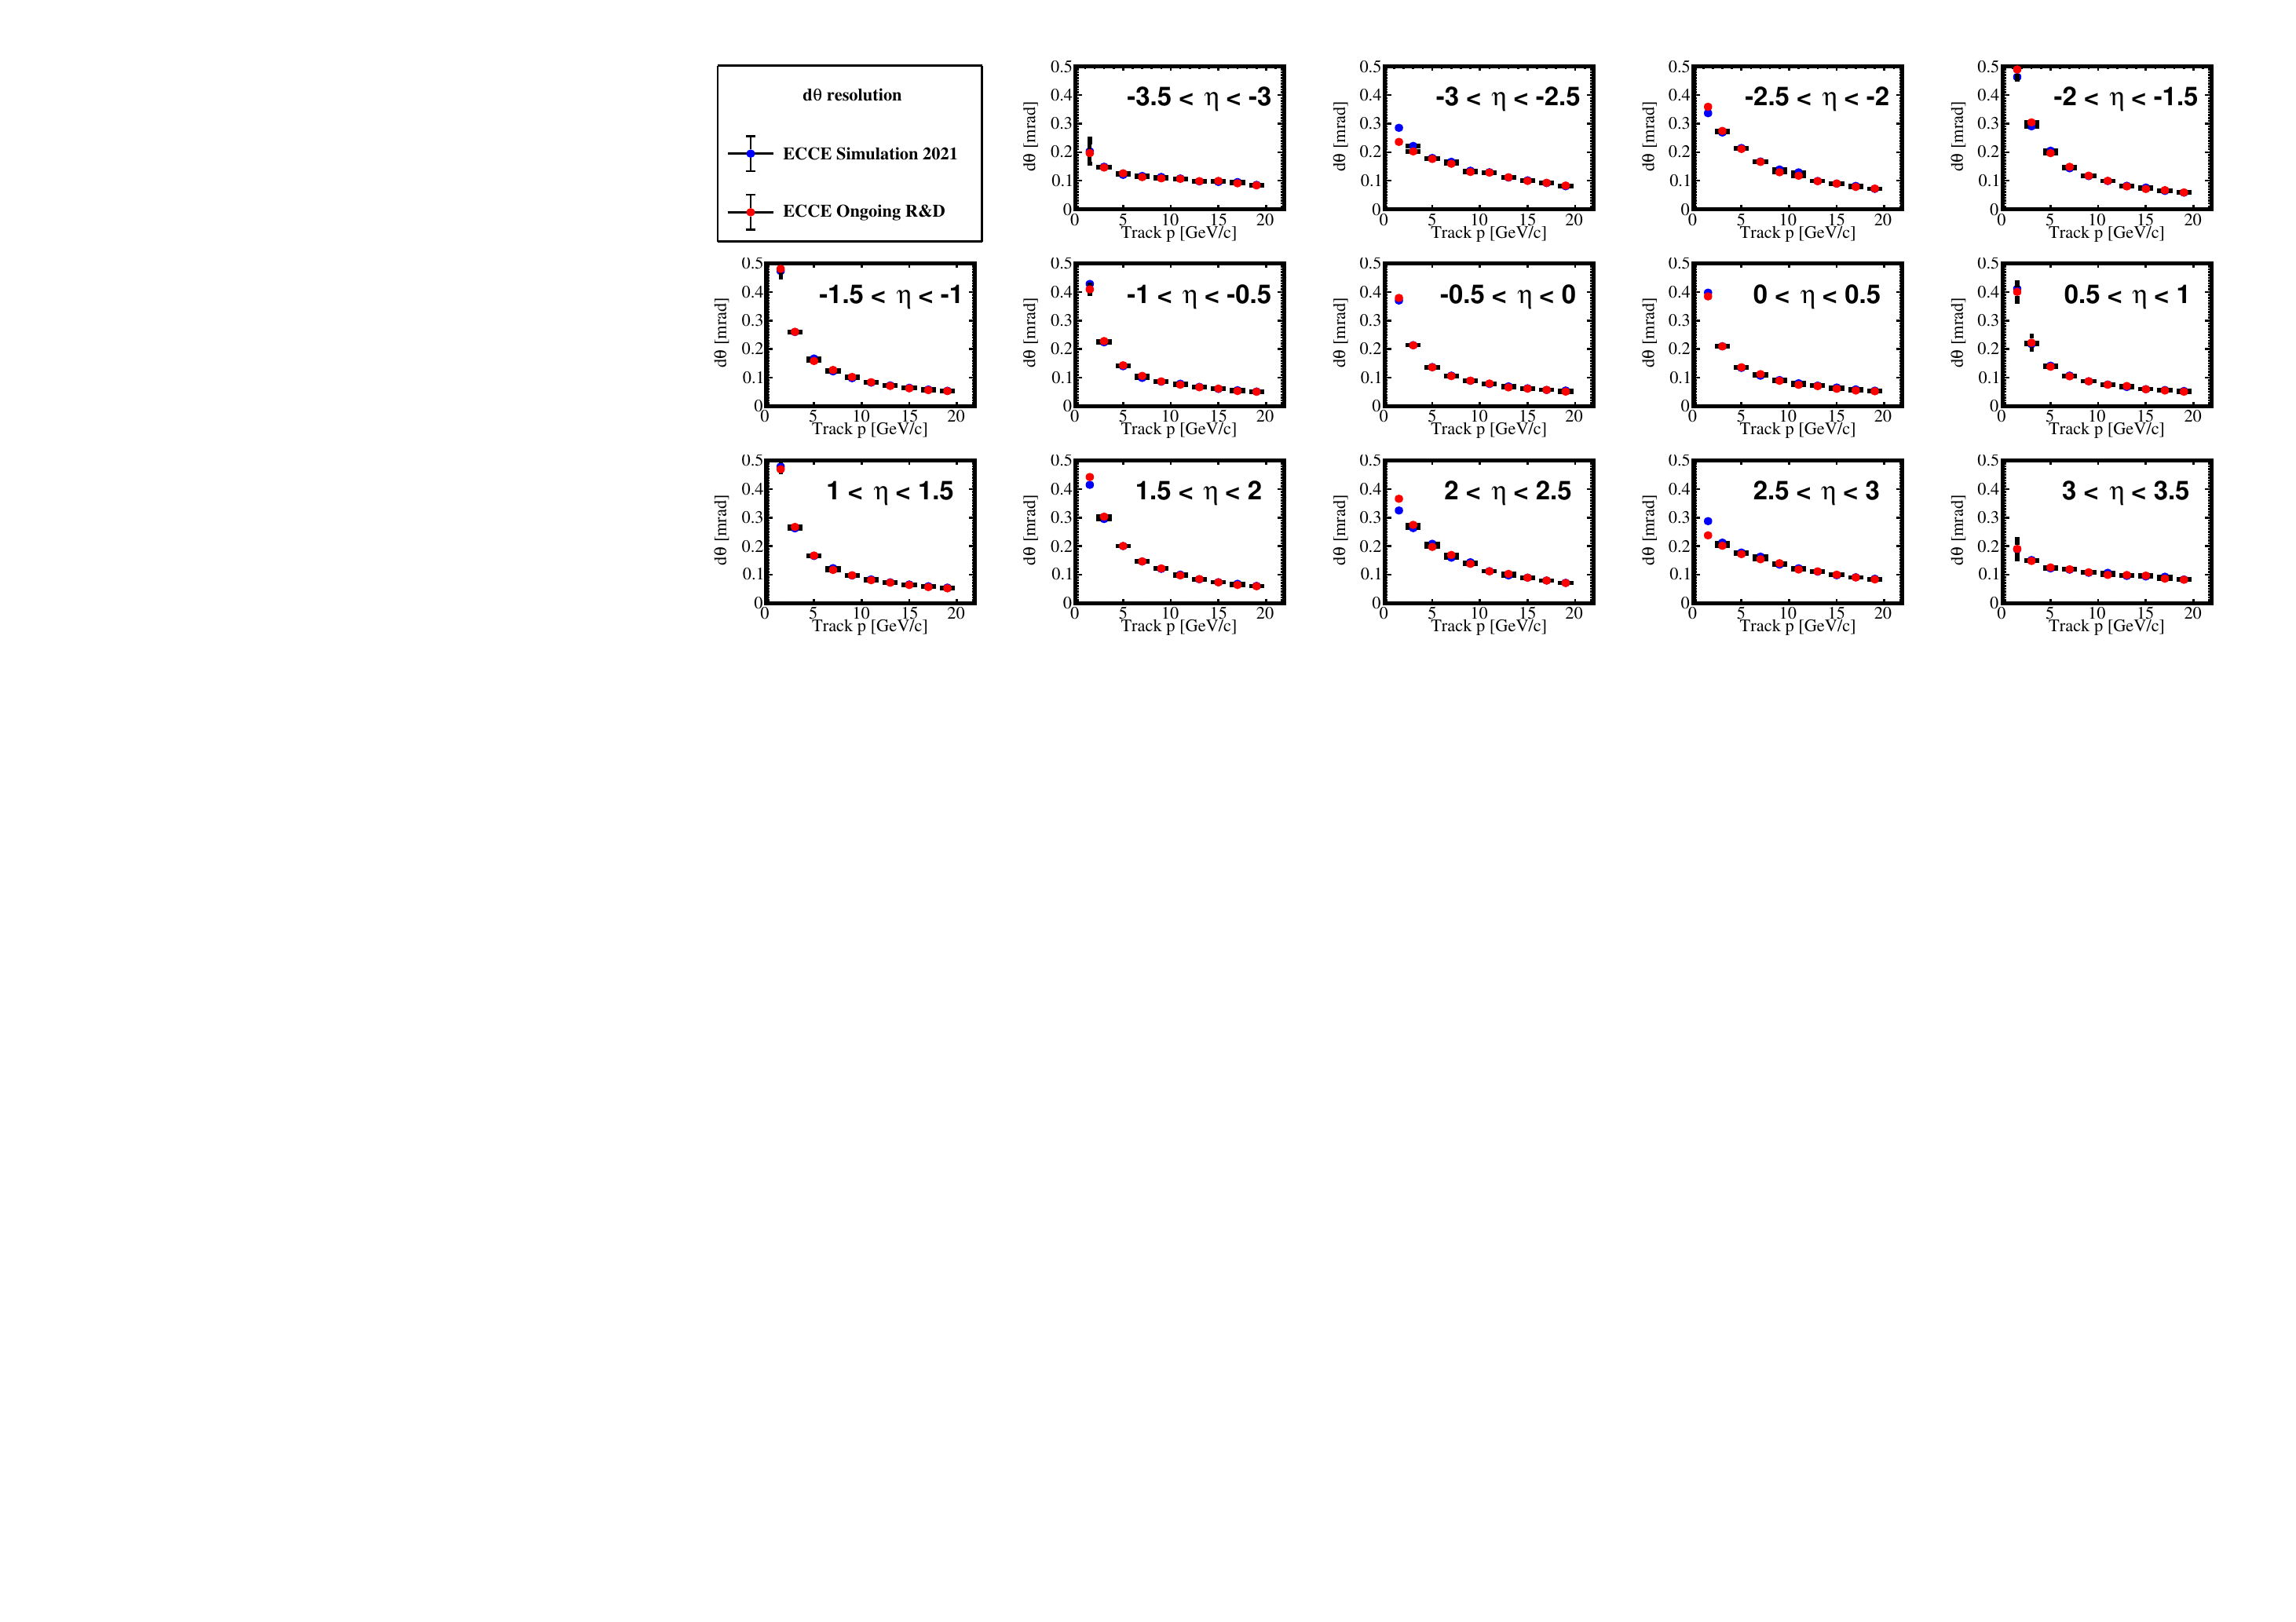}
    \caption{\textbf{Angular resolution ($d\theta$) for ECCE projective geometry and ECCE simulation:} The resolution shows an improvement in the transition region between $1.0 < |\eta| < 1.5$. These plots have been produced using double-Gaussian fits.
    \label{fig:Phase-II_dth_res}
    }
\end{figure*}

\begin{figure*}[!]
    \centering
    \includegraphics[width=0.98\textwidth]{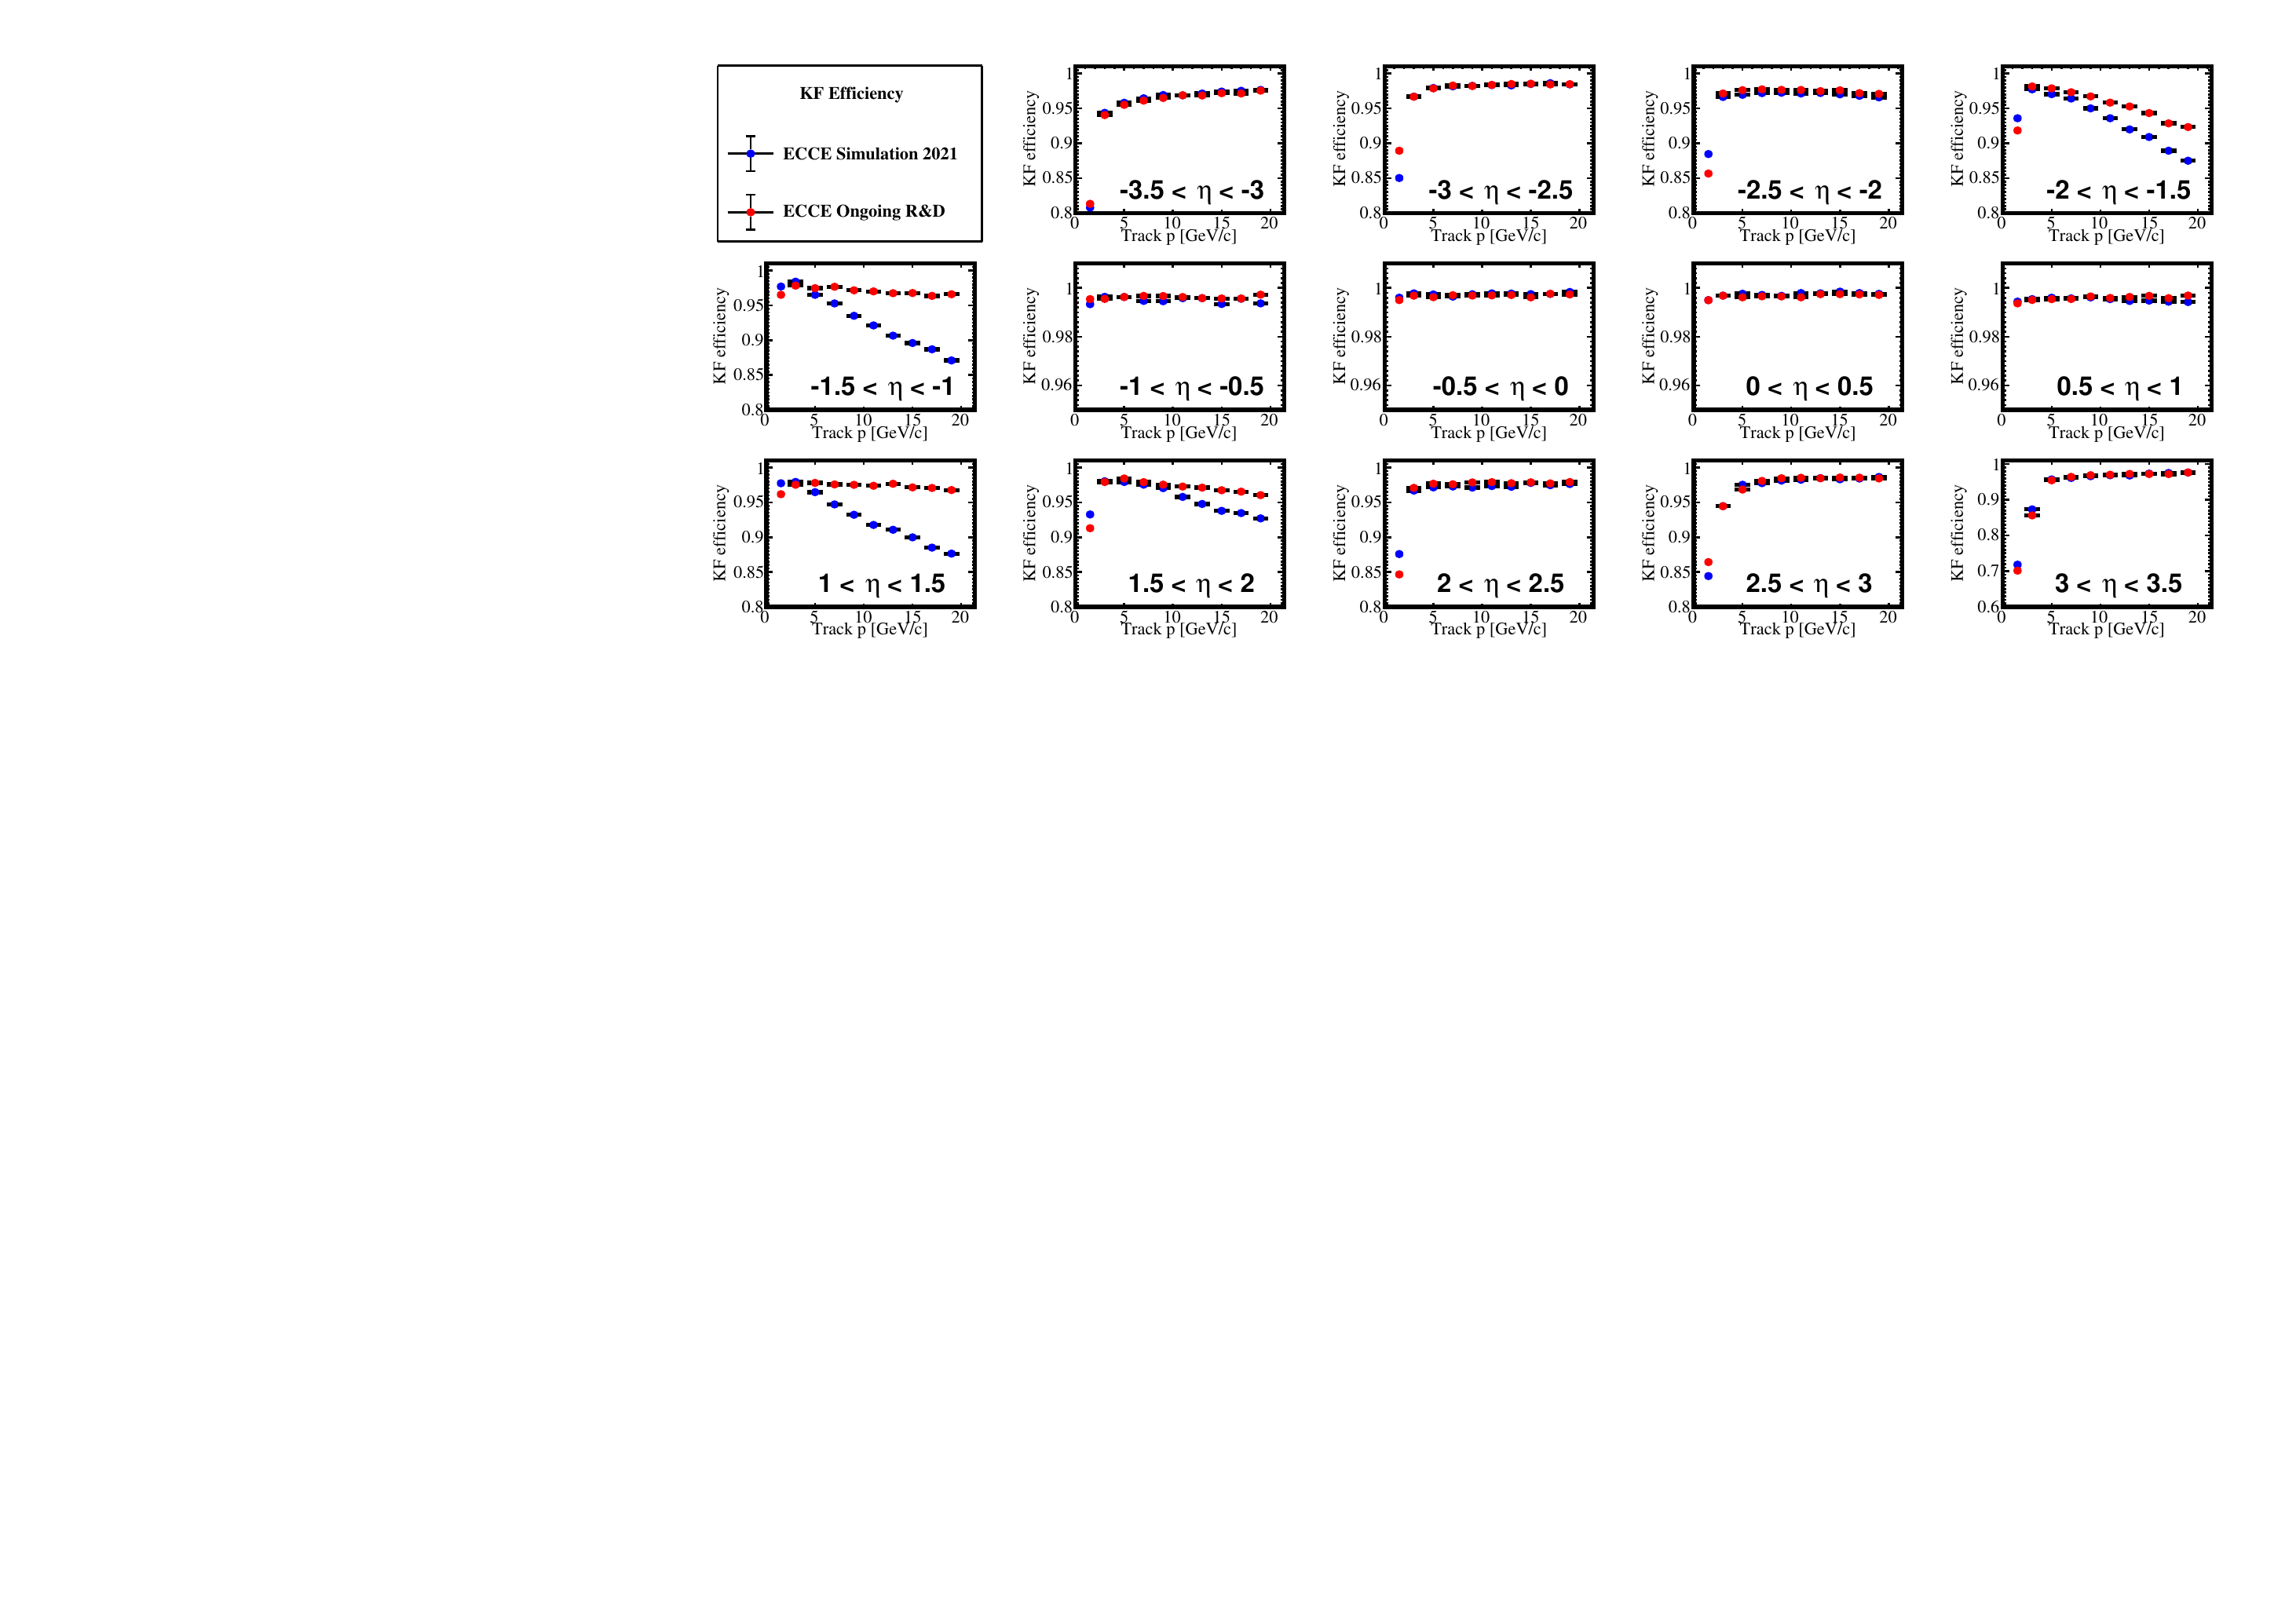}
    \caption{\textbf{KF Efficiency for ECCE projective geometry and ECCE simulation:} Reconstruction efficiency shows an improvement in the transition region between $1.0 < |\eta| < 1.5$. There is a significant drop in the transition region caused due to multiple scattering of the support structure. }
    \label{fig:Phase-II_KF_eff}
\end{figure*}
%\end{comment}

%%%%%%%%%%%%%%%%%%%%%%%%%%%%%%%%%%%%%%%
\subsection*{Validation}\label{subsec:validation}
%%%%%%%%%%%%%%%%%%%%%%%%%%%%%%%%%%%%%%%

Validation is performed by looking at figures of merit that are not used during the optimization process. 
In Sec.~\ref{subsec:physics_analysis} we already described a physics analysis with SIDIS events that further consolidates our conclusions.
We show here additional examples of validation: Fig.~\ref{fig:Phase-II_dph_res} and Fig.~\ref{fig:Phase-II_recon_eff} display the azimuthal angular resolution and the reconstruction efficiency obtained for both the non-projective and the projective tracker designs.
The azimuthal resolution looks consistent within the uncertainty while the reconstruction efficiency looks in general better for the projective design, particularly in the 1 $<$ $|\eta|$ $<$ 1.5 region where the non-projective design has a larger dead area that affects the reconstruction of tracks.

%--------------
%\begin{comment}
\begin{figure*}[!]
    \centering
    \includegraphics[width=0.98\textwidth]{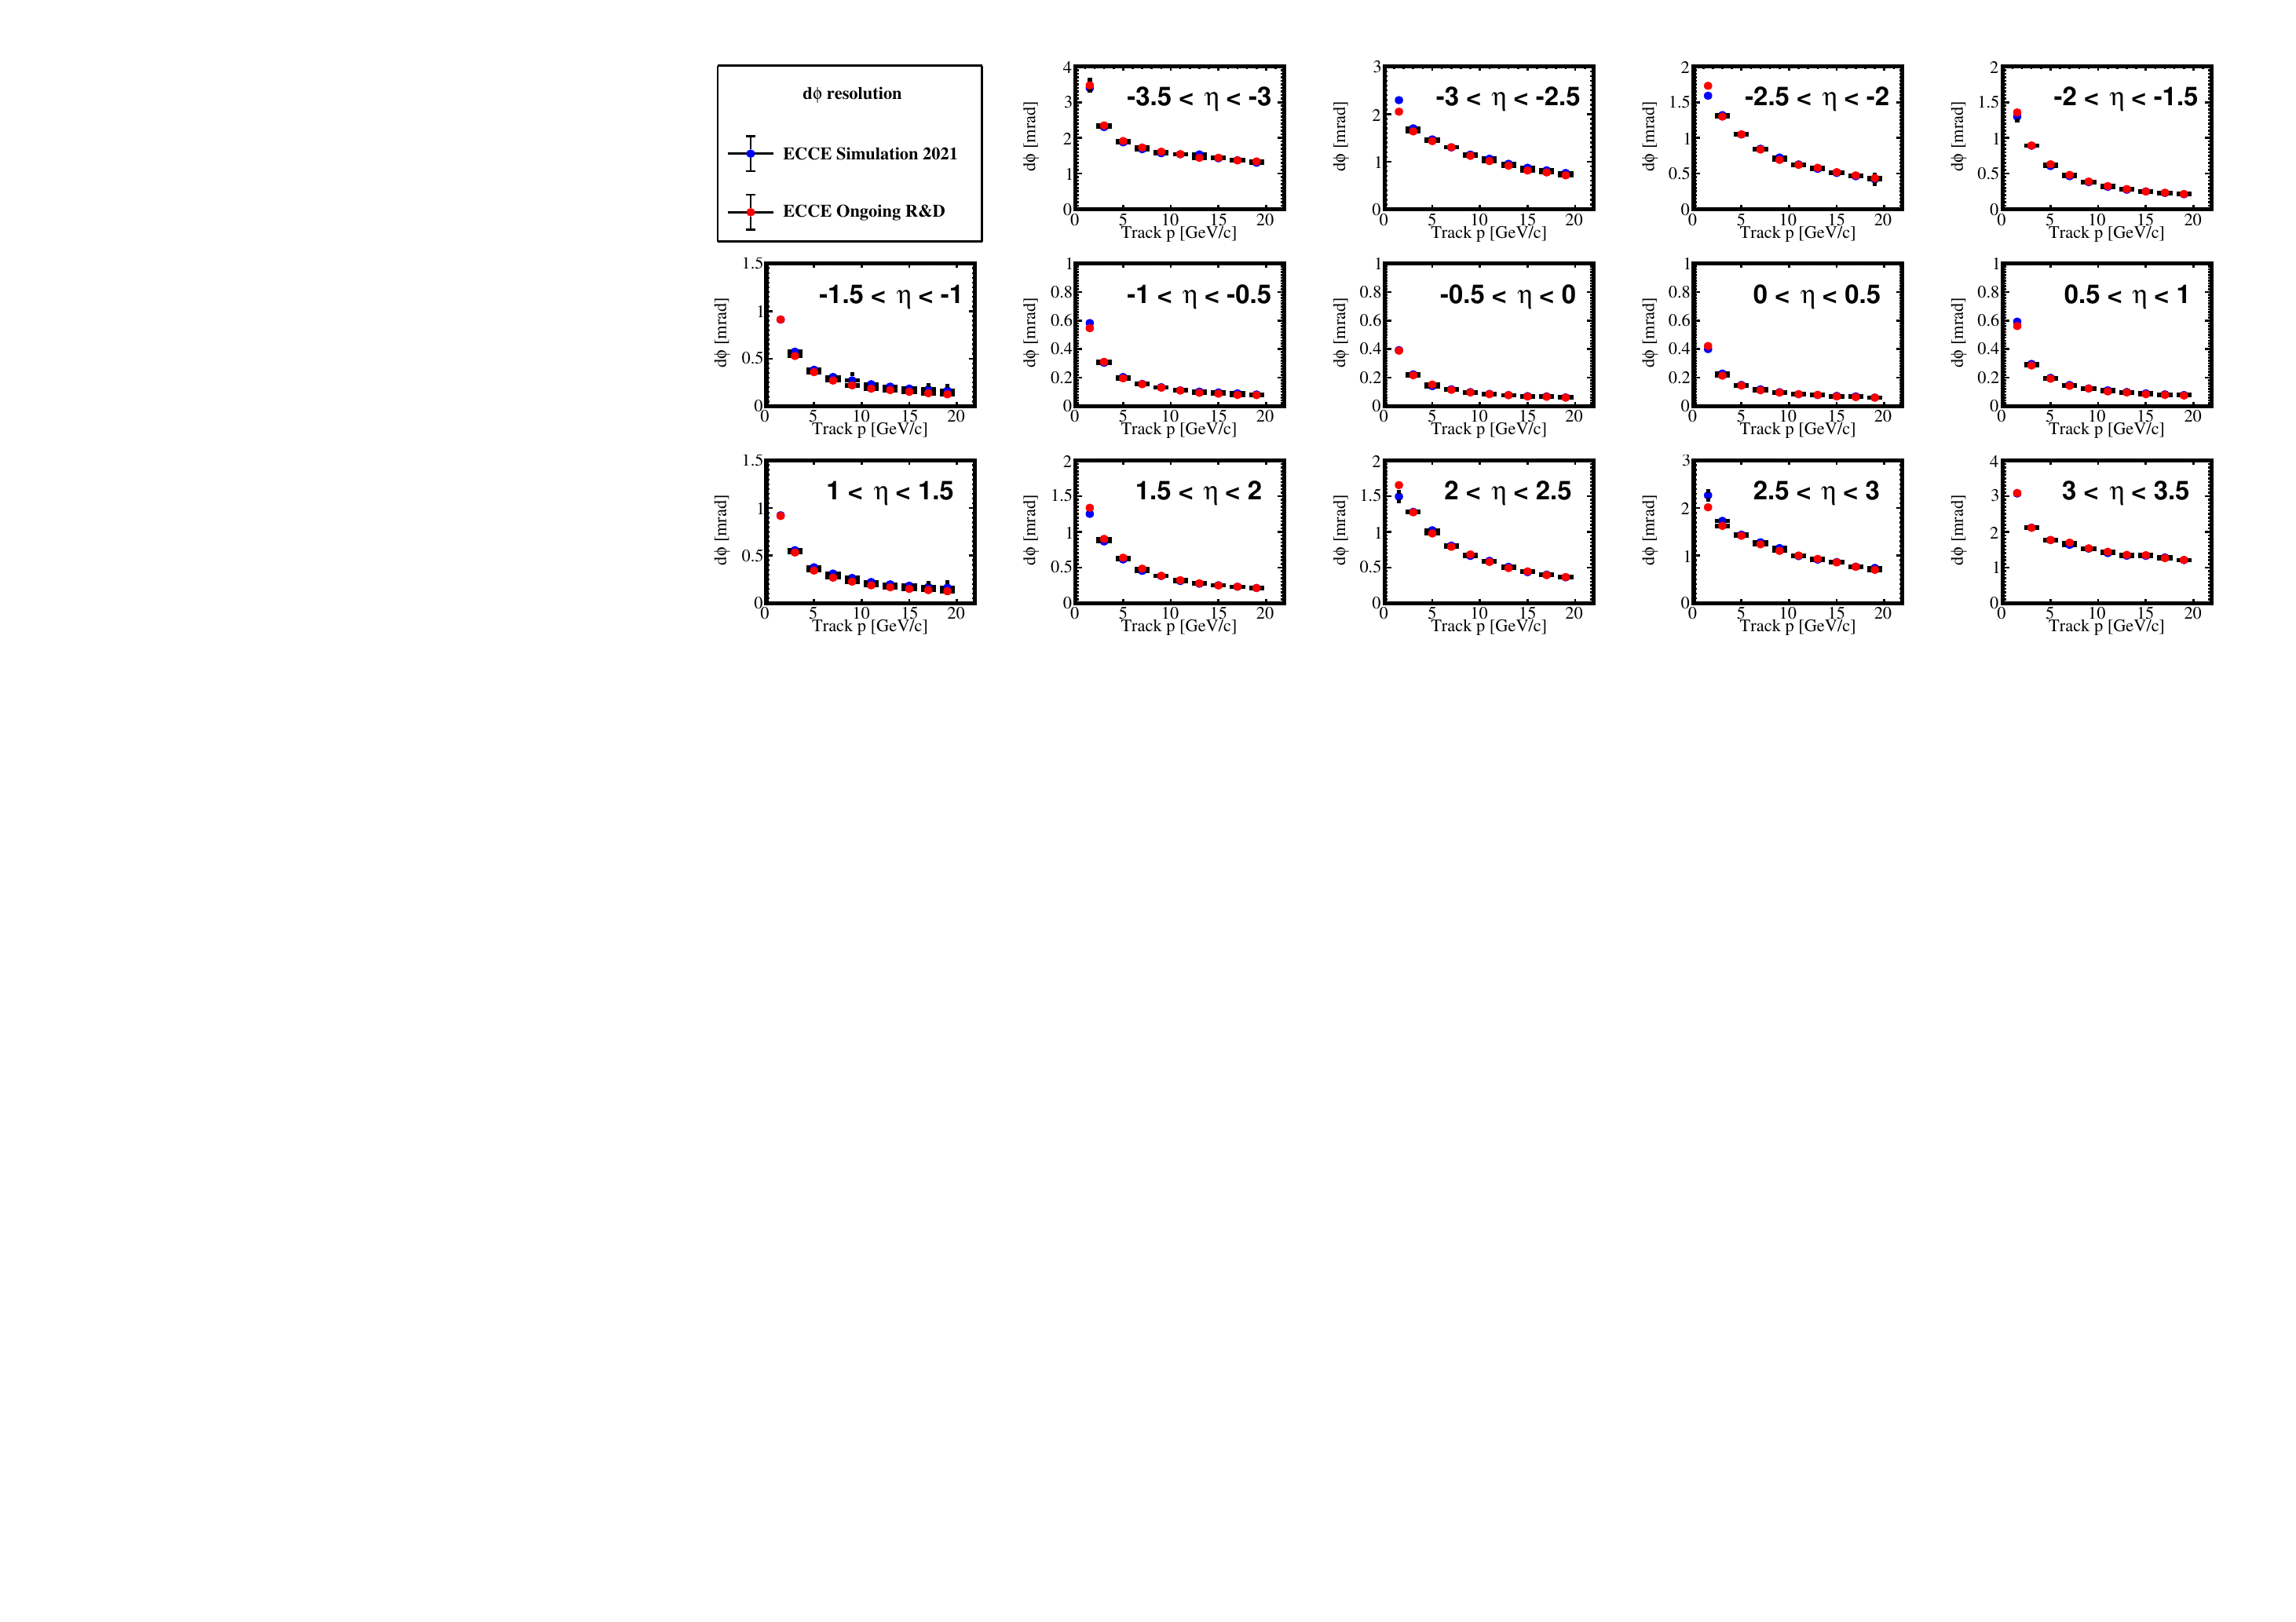}
    \caption{\textbf{Angular resolution ($d\phi$) for ECCE projective geometry and ECCE simulation:} The resolution shows an improvement in the transition region between $1.0 < |\eta| < 1.5$. These plots have been produced using double-Gaussian fits.}
    \label{fig:Phase-II_dph_res}
\end{figure*}

\begin{figure*}[!]
    \centering
    \includegraphics[width=0.98\textwidth]{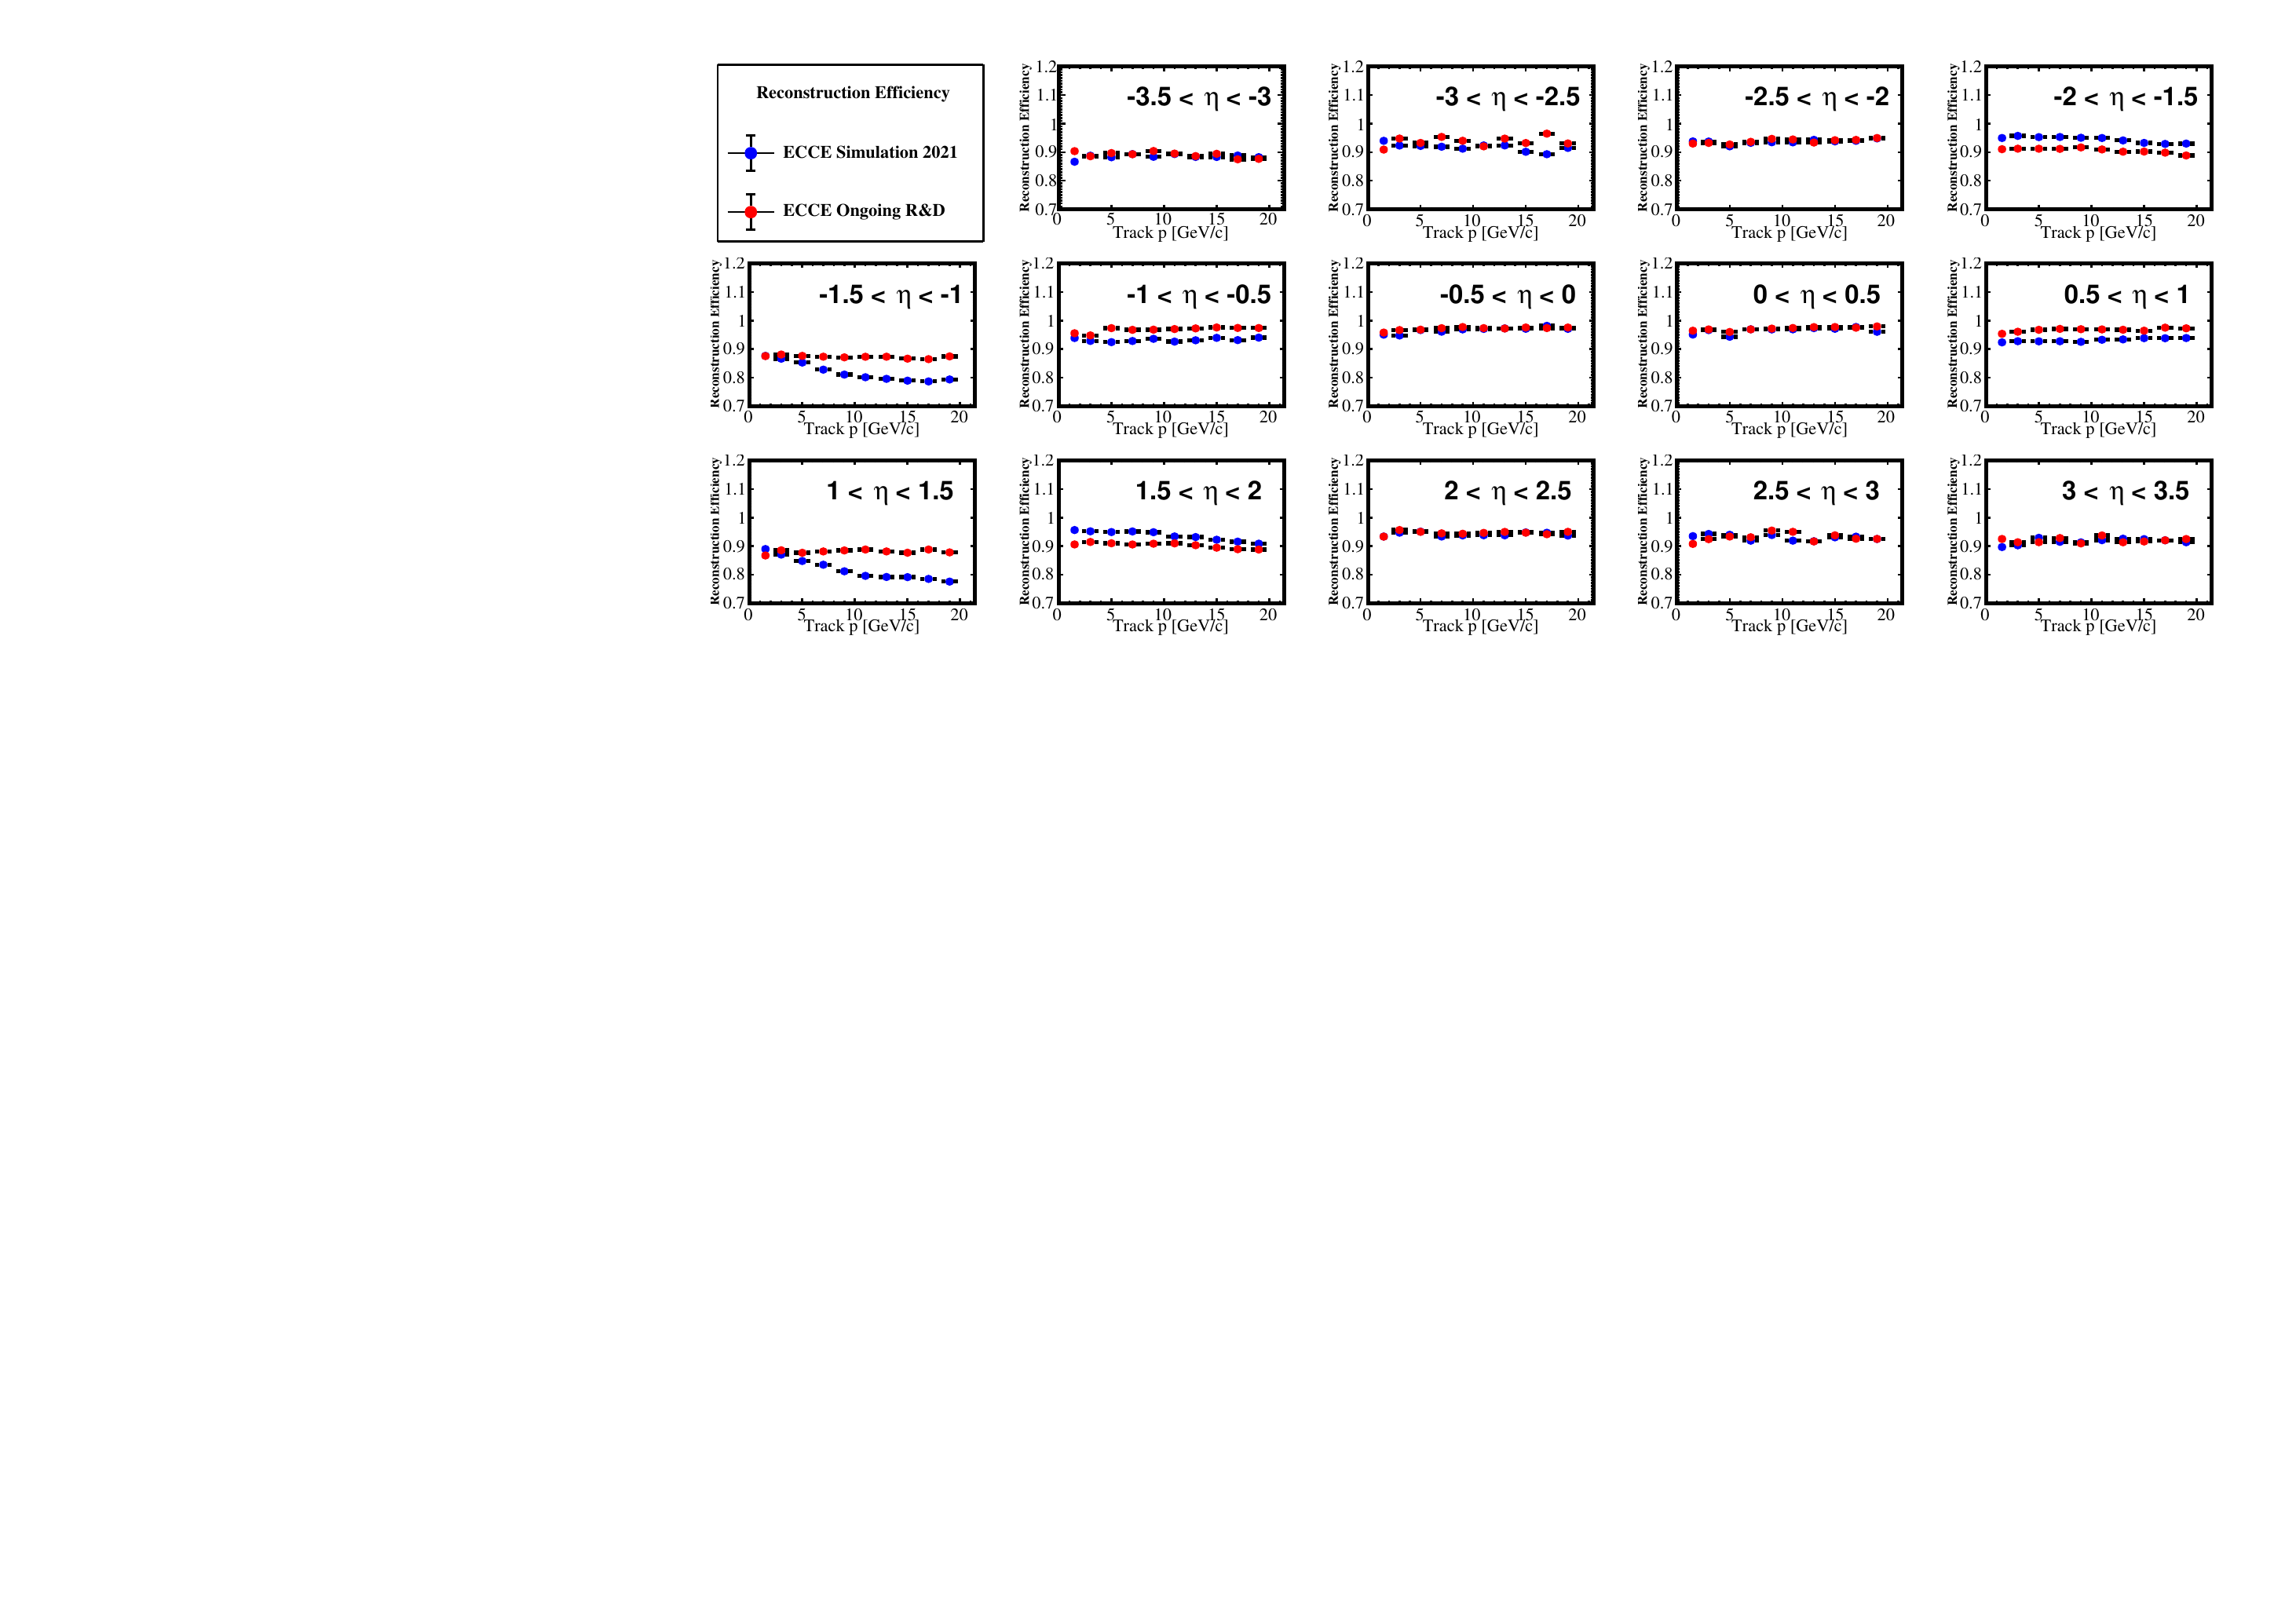}
    \caption{\textbf{Reconstruction efficiency for ECCE projective geometry and ECCE simulation:} Reconstruction efficiency shows an improvement in the transition region between $1.0 < |\eta| < 1.5$}
    \label{fig:Phase-II_recon_eff}
\end{figure*}
%\end{comment}

A comparison between the non-projective and projective designs of the inner tracker is also shown in Fig.~\ref{fig:tracking_projective}, where the projective design concentrates the material in a smaller dead area resulting in better resolution on a wider range of the pseudorapidity.
%

%\begin{comment}
\begin{figure*}[!]
\centering
    \centering
    \includegraphics[width=0.3\textwidth]{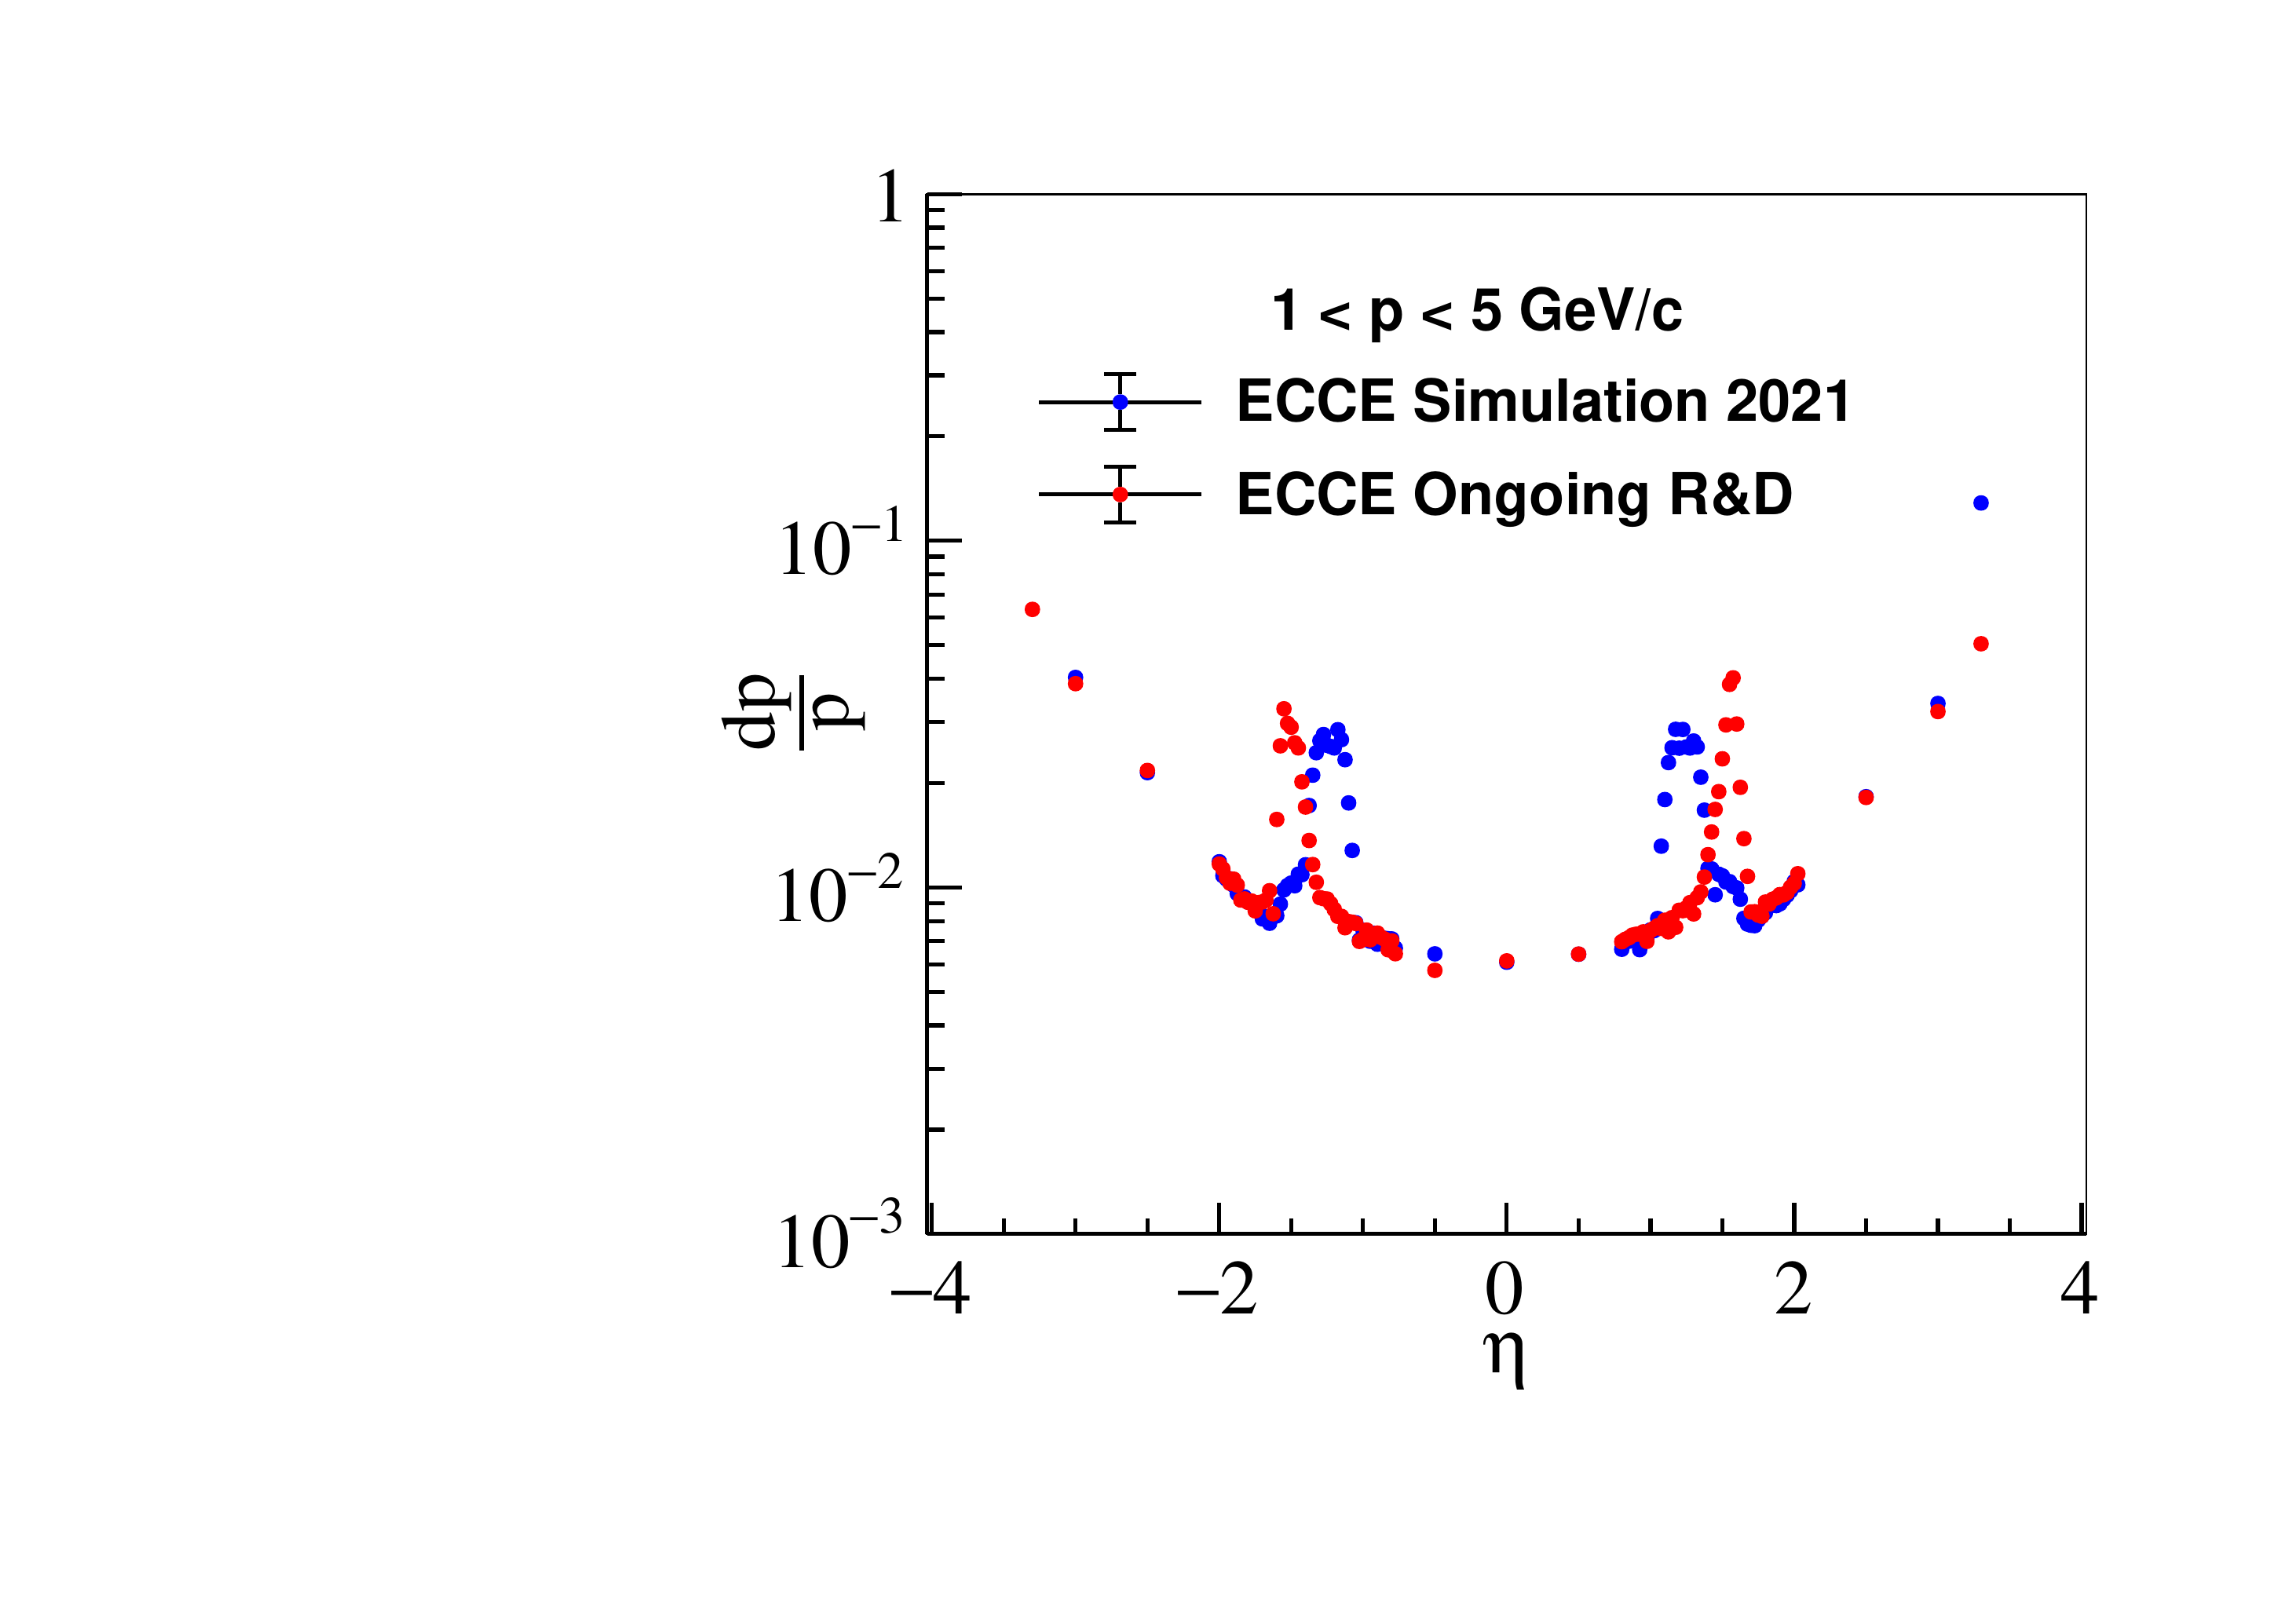}
    \includegraphics[width=0.3\textwidth]{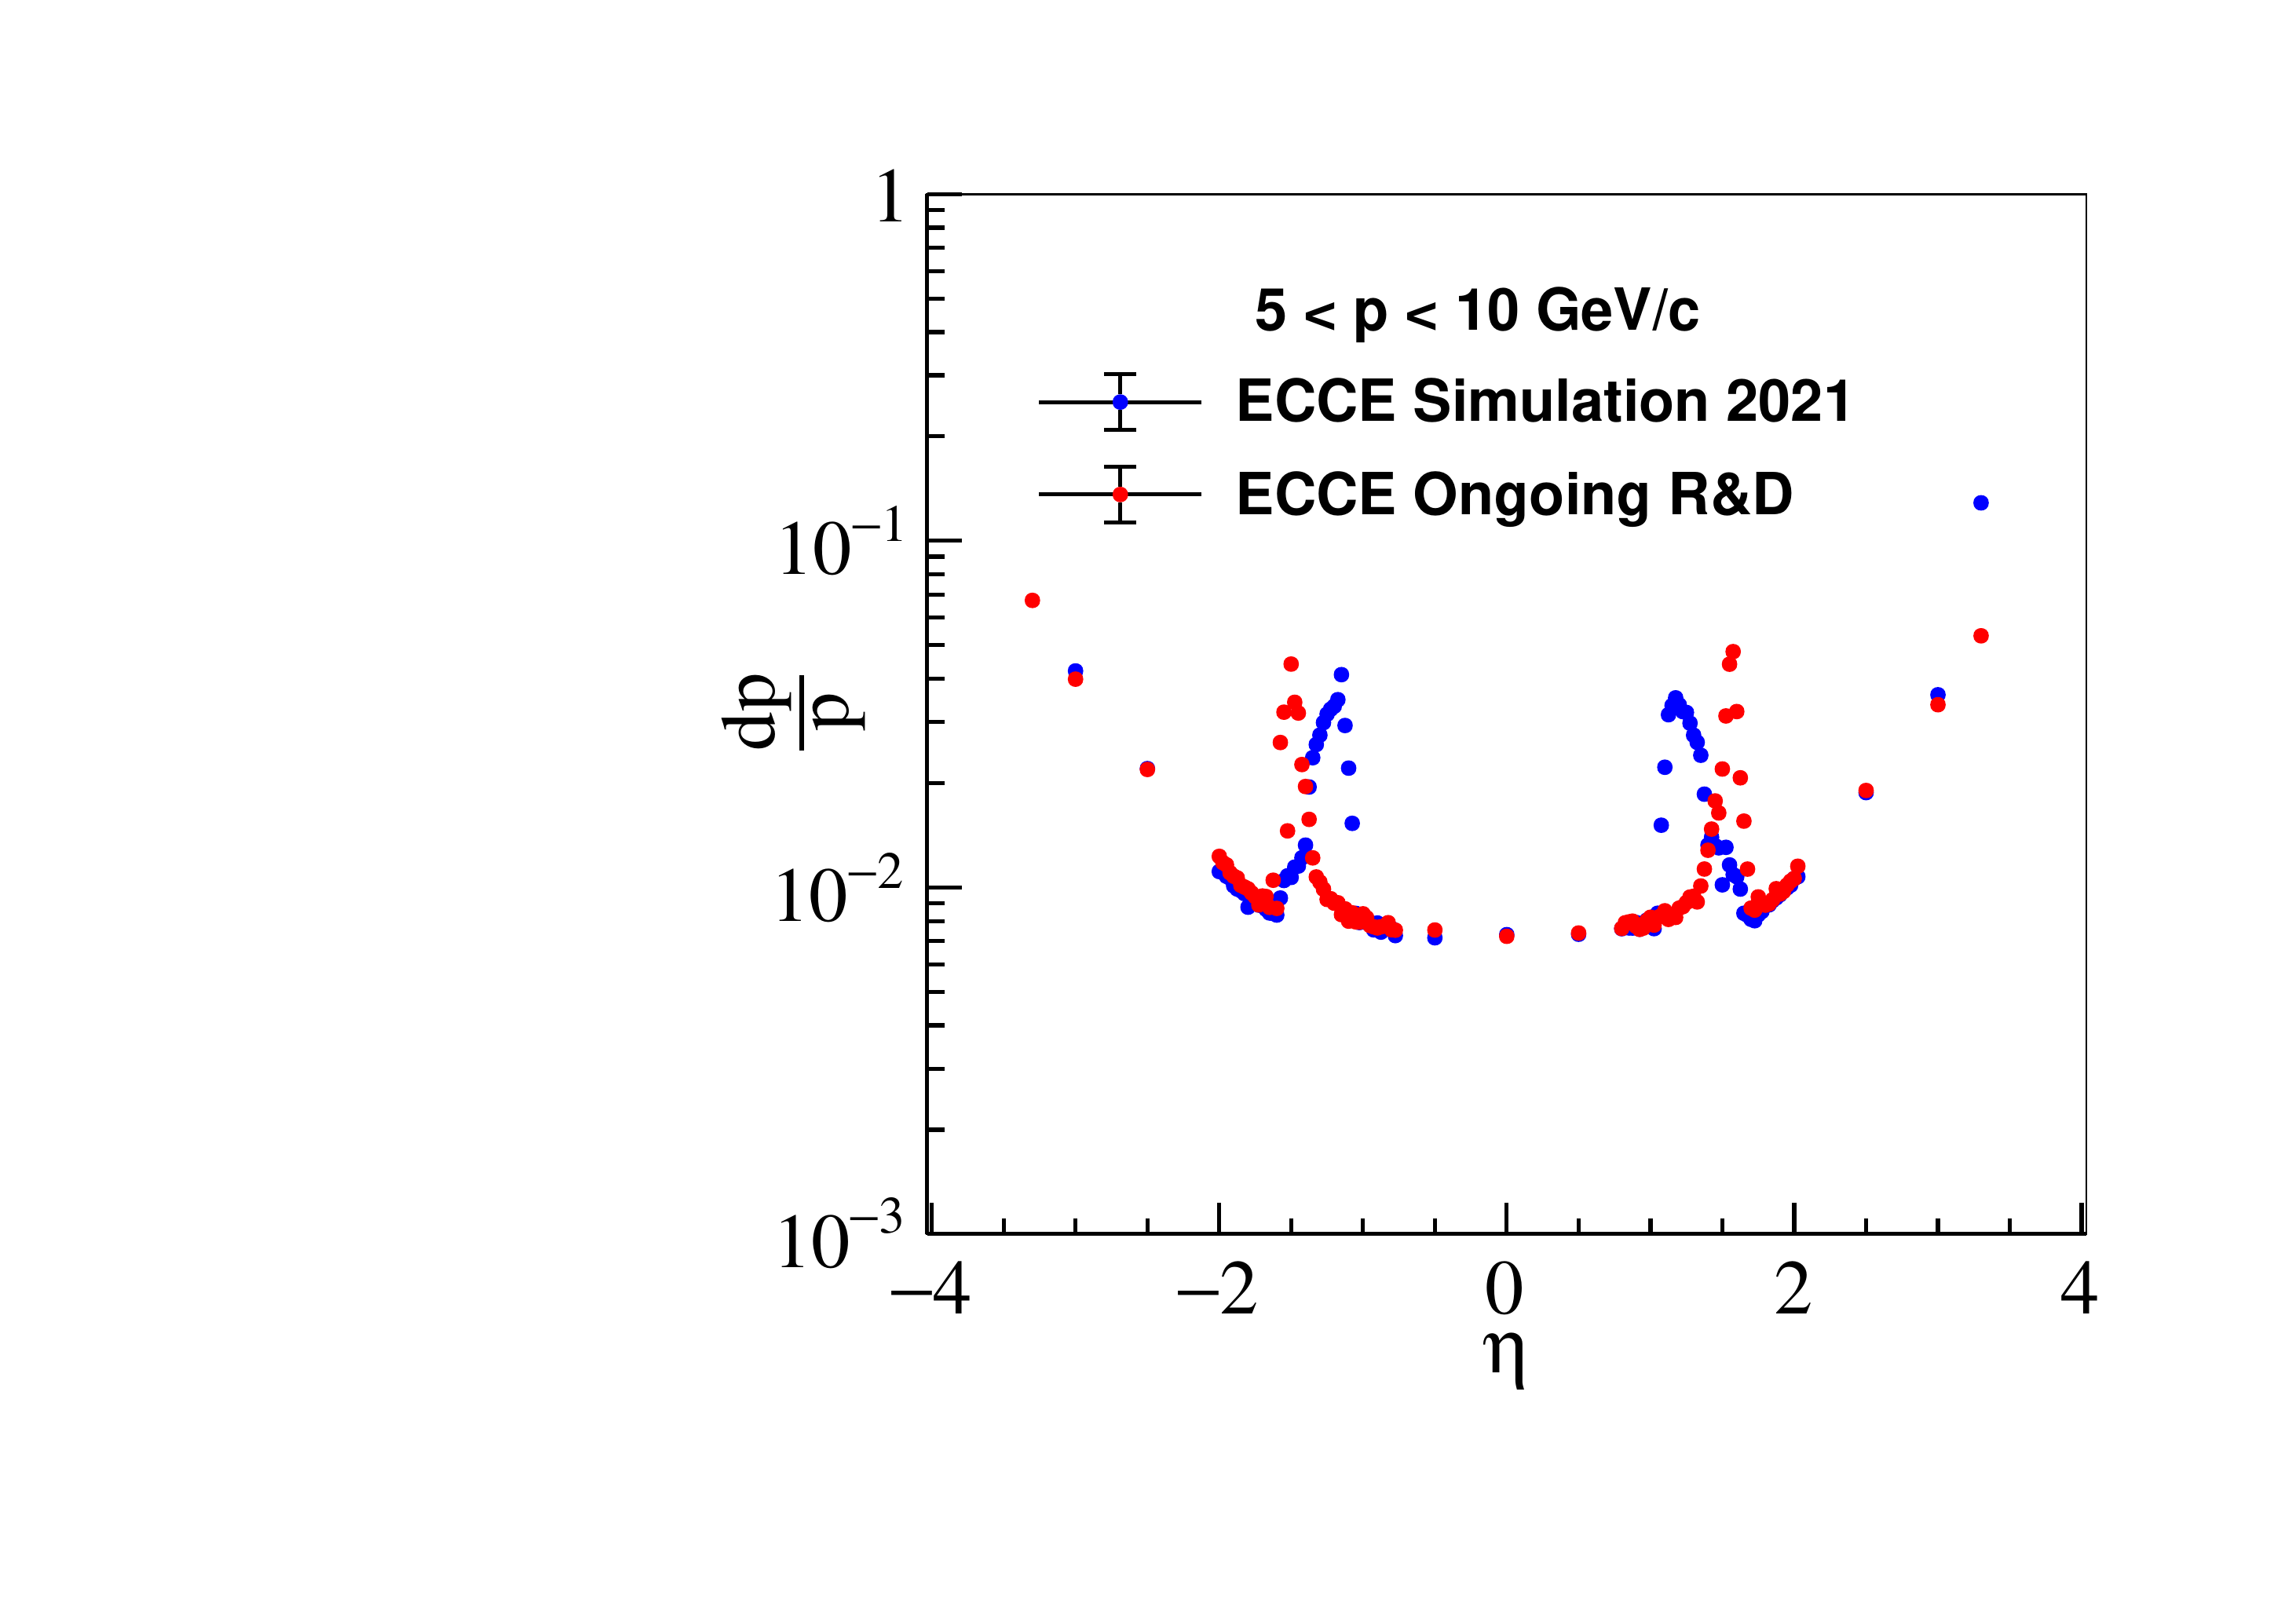}
    \includegraphics[width=0.3\textwidth]{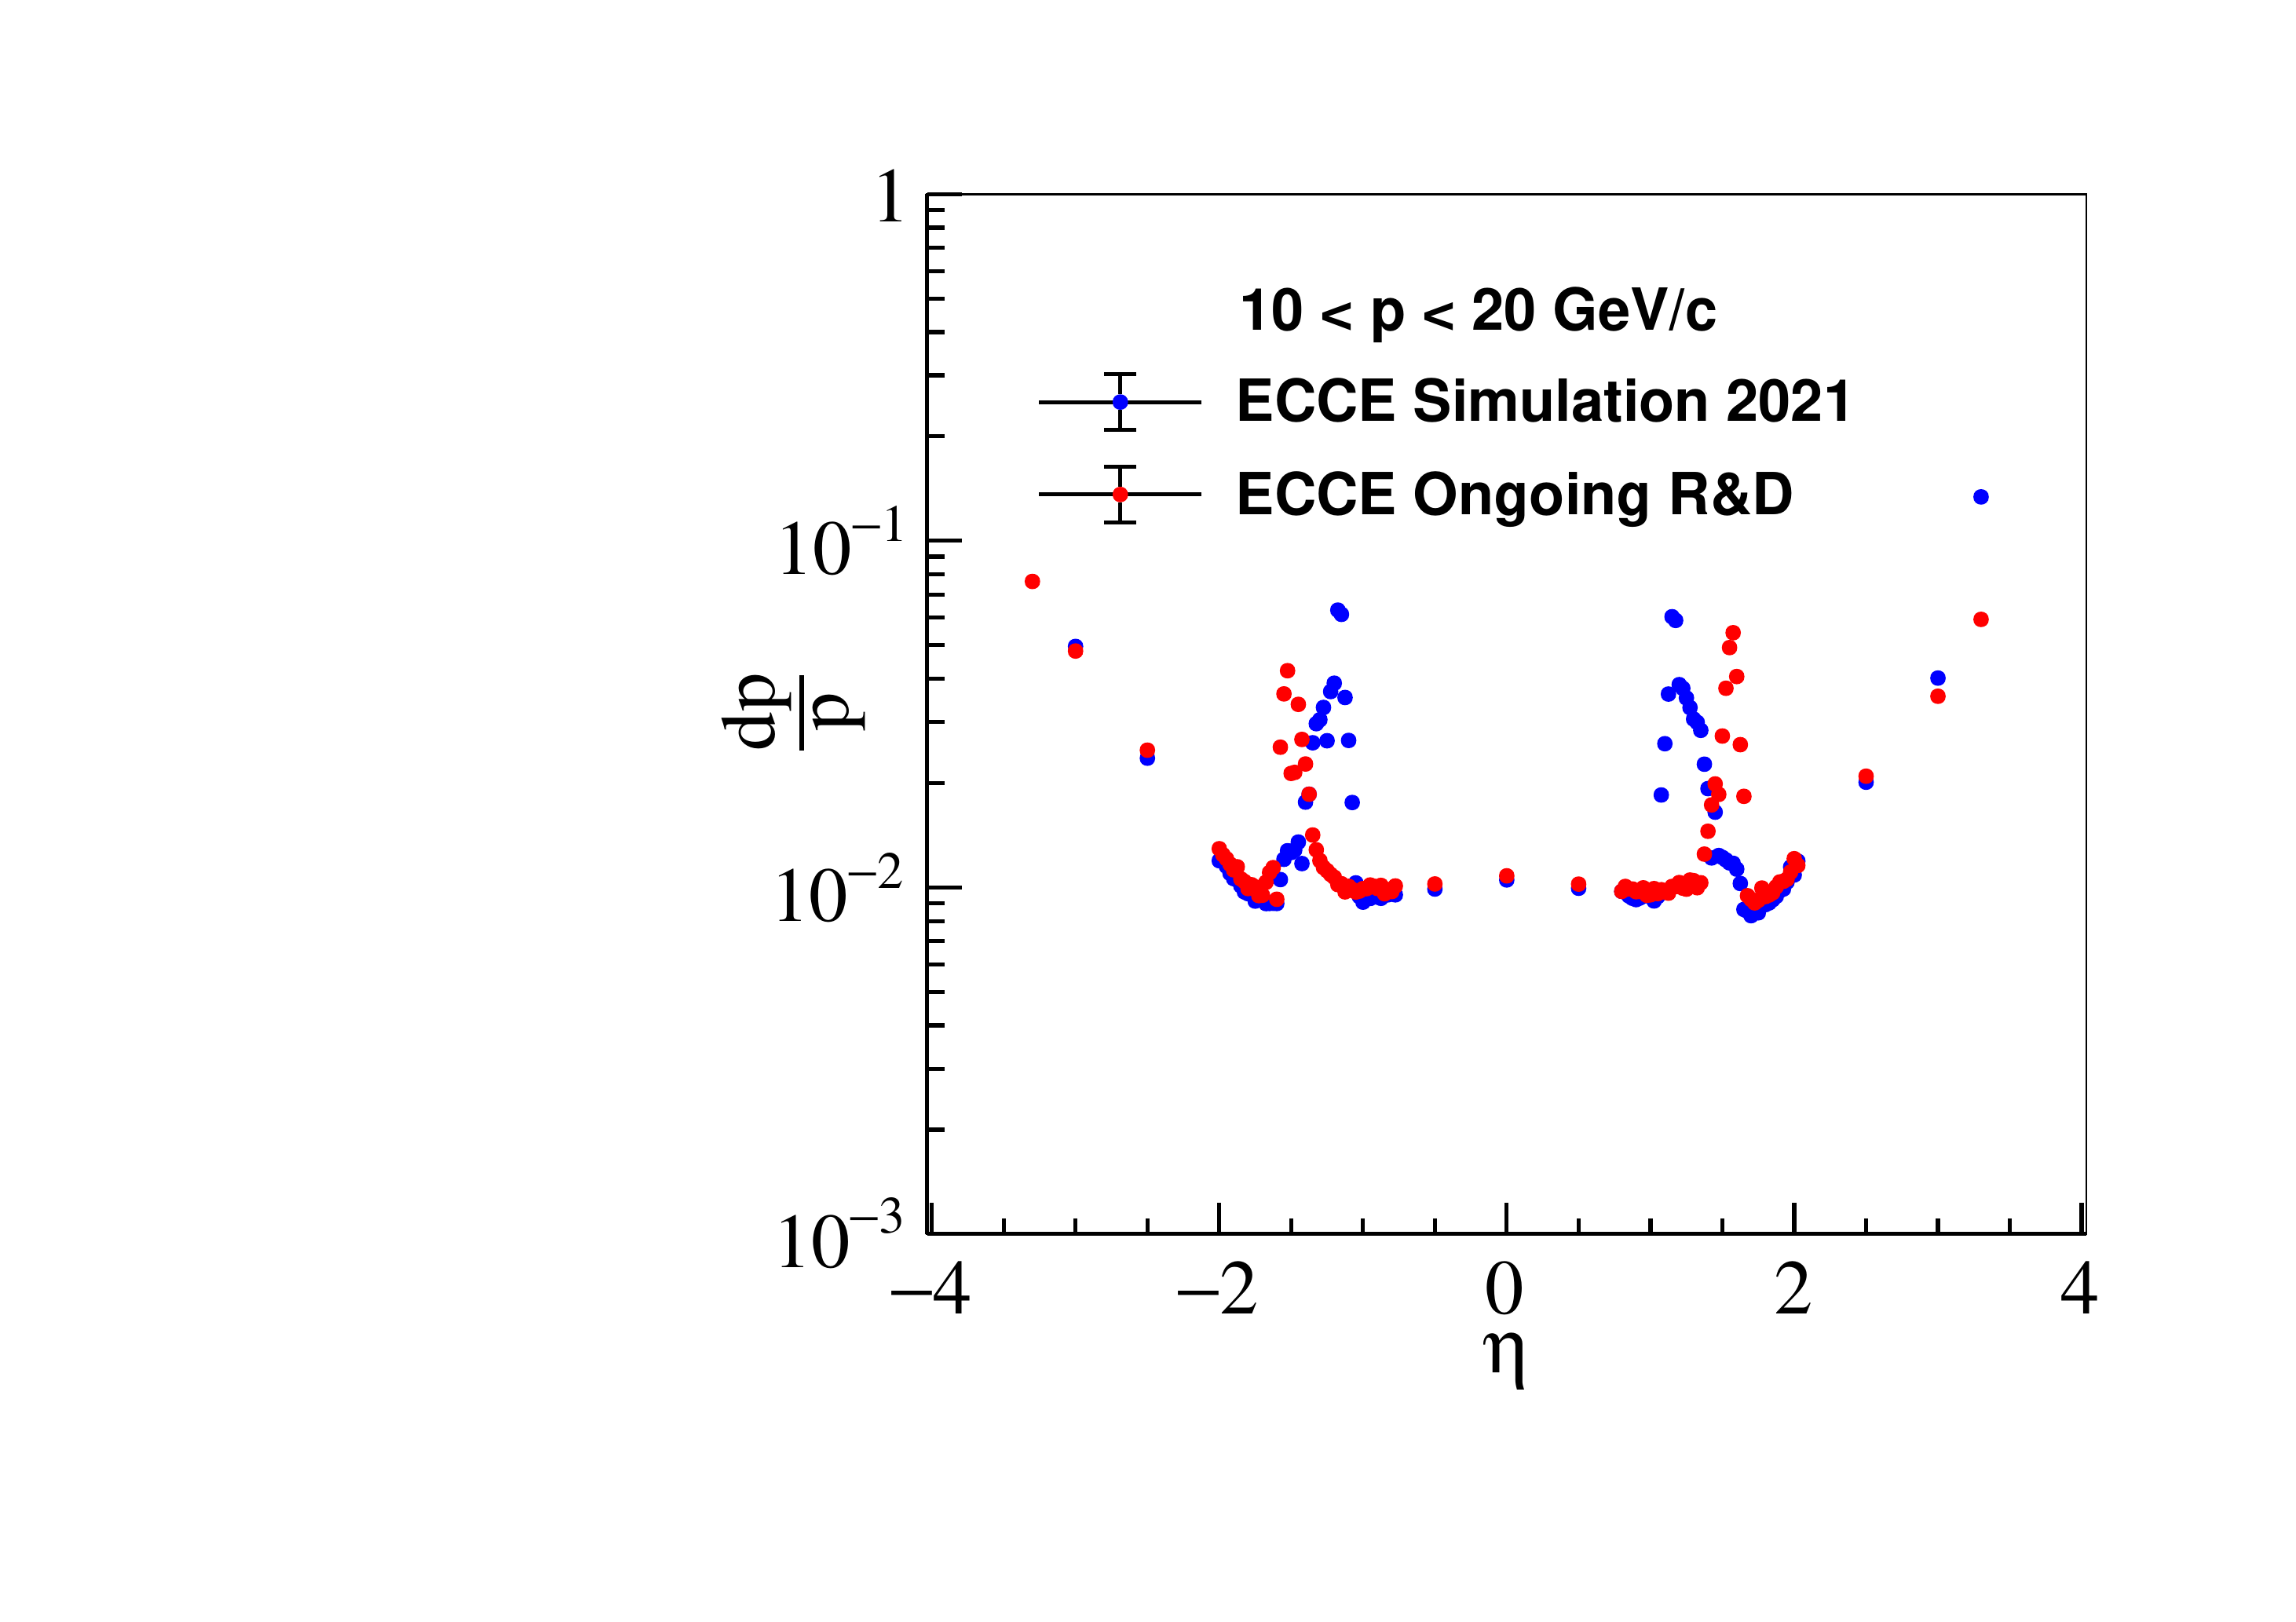}
    \caption{\textbf{Comparison between non-projective and projective inner tracker:}  a comparison in momentum resolution as a function of the pseudorapidity $\eta$ between the non-projective and the projective designs in three bins of momentum. The projective design concentrates the material in a smaller dead area resulting in better resolution on a wider range of the pseudorapidity. %Both designs have been assisted by AI. 
    %\cris{This is going to change into a row with multiple sub-figures (corresponding to bins in momentum); remember to reference this figure in the text.}
    }
    \label{fig:tracking_projective}
\end{figure*}
%\end{comment}
