# Supplementary material for: Quantitative Analysis of Community Evolution in Developer Social Networks Around Open Source Software Projects
Source: arXiv:2205.09935 source file (2022-05-20)
Supplement: Supplementary file 2 [file Appendix_parametrization.tex]

\section{Details on Parametrization}\label{app:par_tracking}

%%%%%%%%%%%%%%%%%%%%%%%%%%%%%%%%%%%%%%%
\subsection*{Tracking System Parametrization} 
%%%%%%%%%%%%%%%%%%%%%%%%%%%%%%%%%%%%%%%

%\cris{Add references for each detector? Reference ECCE detector paper.}

\paragraph{Vertex layers} 
There are three vertex barrel layers in the ECCE tracking system made of MAPS technology. % (ITS3).  already defined
The vertex cylinder consists of strips which are made of pixels, where the individual sensor unit cell size is 17.8 mm $\times$ 30.0 mm.
The length of the vertex layers is fixed at 27 cm; %\cris{(30) drop?}
the radii of the three vertex layers are fixed to 3.4, 5.67, 7.93 cm, respectively.
For the non-projective design, the angle of the support structure with respect to the interaction point is fixed ($\theta = 36.5\degree$) and the radius of the support is at 6.3 cm, while the length of it is 17 cm.
For the projective design, the radius of the support structure is the same, while the length is calculated based on the angle of projection and the radius as shown in Fig.~\ref{fig:SupportStructureparametrization}.

\paragraph{Sagitta layers} 
There are two sagitta barrel layers in the ECCE tracking system.
The sagitta barrel layers are made of MAPS technology and have 
%
%The sagitta barrel layer has a 
fixed length of 54 cm.
For the non-projective design the radii of the sagitta layers are 21.0, 22.68 cm, respectively. For the projective parameterization,the radius of the sagitta barrel is calculated such that there are no gaps in the acceptance of the region enclosed by the barrels, according to the following equation:
%. The radius of the barrel layer is calculated as: 
$$r_{sagitta} = \frac{l_{sagitta}}{2}\tan{\theta}.$$

The radius of the sagitta layers is also constrained since the strips have fixed width  $w$ = 17.8 mm; therefore we want to minimize the quantity: 
%
%$$\frac{2 \pi r_{sagitta}}{1.78} = n; n \in \mathbb{Z}^{+}.$$
%
$$ min \Bigg\{ \Bigg| \frac{2 \pi r_{sagitta}}{w} - \floor*{\frac{2 \pi r_{sagitta}}{w}} \Bigg| \Bigg\},$$
 where $\floor*{x}$ represents the ceiling of x.

\paragraph{$\mu$Rwell layers}
In the ECCE tracking system there are three cylindrical $\mu$Rwell layers, each %end of each %$\mu$Rwell barrel layers.
 endowed with a support ring.  
An extended supporting plateau is included at either ends of the $\mu$Rwell to rest the entire cylindrical detector on this platform. 
This results in a constant shift of the support cone by the plateau length (5 cm) as shown in Fig.~ \ref{fig:SupportStructureparametrization}.
%
%Therefore, for each $\mu$Rwell layer the support cone is shifted constantly by the length of the plateau.
%
For both the non-projective design and the projective design the $\mu$Rwell-1 radius is a free parameter. The length of the $\mu$Rwell-1 is calculated based on the angle of the conical support structure. 
In the non-projective design we have the conical support structure angle fixed ($\theta = 36.5\degree$), therefore the length of $\mu$Rwell-1 depends only on its radius; $\mu$Rwell-2 has its radius as a free parameter;
since the angle of the conical support structure is fixed the length of $\mu$Rwell-2 depends on its radius. 
%The optimization always preferred to maximize the radius and therefore was fixed in the projective design.  
%
 In the projective design instead the $\mu$Rwell-2 has a fixed radius of 51 cm ($i.e.$, $r_{max} +$ 1 cm). The length of the $\mu$Rwell-2 is calculated based on the angle of the conical support structure. The length of the $\mu$Rwell takes into account the constant shift due to the plateau.  
The dimensions of $\mu$Rwell-3 are fixed in both non-projective and projective designs; the $\mu$Rwell-3 is outside of the inner tracking system and it has radius of 77 cm and a total length is 290 cm.

\paragraph{EST/FST disks}
%

%The FST/EST disks are made of MAPS technology (ITS3). 
%The disks are tiled up using MAPS pixel which comes in fixed dimension of 17.8 mm $\times $ 30.0 mm; we already said this
%
For both the non-projective and projective designs, 
$R_{min}$ of the disks must be compatible with the beam pipe envelope which increases in radius as a function of $z$; 
$R_{out}$ of the disks is parametrized to be compatible with the support cone structure shown in Fig. \ref{fig:SupportStructureparametrization} which has an angle $\theta$ that is variable in the projective design and fixed in the non-projective case. 
For the non-projective design, the $z$ positions of the disks were all free parameters in the first optimization pipelines. However, to maximize the hit efficiency, some disks have been eventually placed within the support cone at the beginning of every plateau (Fig. \ref{fig:SupportStructureparametrization} with fixed angle $\theta = 36.5\degree$). Therefore, two disks in the electron-going direction and two disks in the hadron-going direction are not free to vary in $z$. 
For instance, consider Fig.~\ref{fig:ECCE_Tracking_non_proj_and_proj} (right), where EST3, EST4, FST3, FST4 are placed at the begin of the pleateau, whereas the disks EST1, EST2, FST1, FST2, FST5 are free to vary in $z$ position.
The same parameterization is extended to the projective design and made compatible with a varying conical support structure.

As the disks are tiled up using MAPS pixels, the difference between $R_{min}$ and $R_{out}$ is constrained to optimize the sensor coverage for all disks; this is implemented by means of two functions, namely:
%
%$$(R_{max} - R_{min})/d = n; n \in \mathbb{Z}^{+},$$
%%$$(R_{max} - R_{min})/30.0 = n; n \in \mathbb{Z}^{+}$$
%
% where $d=$ 17.8 or 30.0 mm. 
%
% to account for the constraints in all the FST and EST disks in the end caps region, 
% this is done with two functions (one for $d=$ 17.8,  30.0 mm) are considered, namely:
 $$min \Bigg\{ \sum_{i}^{all \ disks} \Bigg| \frac{R^{i}_{out} - R^{i}_{in}}{d} - \floor*{\frac{R^{i}_{out} - R^{i}_{in}}{d}} \Bigg| \Bigg\},$$
%$$\sum_{i} \Bigg| \frac{R^{i}_{max} - R^{i}_{min}}{30.0} - \text{ int}\Bigg(\frac{R^{i}_{max} - R^{i}_{min}}{30.0}\Bigg) \Bigg| == 0$$
%
%where $\floor*{x}$ represents the ceiling of x. 
 where $d=$ 17.8, and 30.0 mm. 
 This limits the amount of violation made by a design solution. 
%\cris{We should add this is done by adding a constraint function. @karthik: can you add?}

\paragraph{TOF system} 
The central barrel TOF (CTTL) is an AC-LGAD based TOF detector with a fixed radius of 64 cm and a fixed length of 280 cm.
The TOFs at the electron-going endcap (ETTL) and the hadron-going endcap (FTLL) are AC-LGAD-based TOF disks.  
For the non-projective design the TOF detectors have fixed dimensions. 
For the projective design the TOF detectors in the end cap regions have their $z$ positions as free parameters. 
$R_{in}$ and $R_{out}$ of the ETTL/FTTL disks depends on the position of the disk $z$. The $R_{in}$ of the disk should be compatible with the radius of the beam envelope which increases linearly as a function of $z$; $R_{out}$ of the disks varies as a function of $z$ such that the acceptance coverage by the ETTL/FTTL is roughly unaltered.

\begin{comment}
\paragraph{MPGD System \cris{keep here?}}
%
EMPGD and FMPGD are disk-like gaseous detectors placed in the electron-going and in the hadron-going directions, respectively;
%
$R_{min}$ and $R_{max}$ of the EMPGD/FMPGD disk depends on the position of the disk $z$. The $R_{min}$ of the disk must be compatible with the radius of the beam envelope which increases linearly as a function of $z$.
%
$R_{max}$ of the disk varies as a function of $z$ such that the acceptance coverage provided by the EMPGD/FMPGD is roughly unaltered.
\end{comment}

\paragraph{PID Detectors}
The Detection for Internally Reflected Cherenkov light (DIRC) is a detector for PID in the barrel region. DIRC system has fixed dimensions and occupies a radial space from 71.5 cm to 76.6 cm. 
%, see Fig.~\ref{fig:ECCE_TrackingPID_Detailed}.
%
The modular RICH (mRICH) is a Ring Imaging Cherenkov detector system in the e-going direction with fixed dimensions. 
mRICH has a $z$ position starting at -135 cm extending in $z$ to -161 cm.
The dual Radiator Imaging CHerenkov (dRICH) detector is a detector system in the forward direction with fixed dimensions. dRICH has a $z$ position starting at 180 cm and extends up to 280 cm.
\newline
\newline
The thickness of the detectors and support structures are also taken into account to avoid overlaps between the detectors. 
The most recent optimization pipelines were extended to also include in the parametrization the outer tracking layers in the two endcaps, as explained in Sec. \ref{subsec:encoding}.    
An overlap check is performed each time a new design point is evaluated during the optimizaton process.

%%%%%%%%%%%%%%%%%%%%%%%%%%%%%%%%%%%%%%%
\subsection*{Support Structure Parametrization}\label{subsec:par_tracking}
%%%%%%%%%%%%%%%%%%%%%%%%%%%%%%%%%%%%%%%

The implementation of the projective geometry of the inner tracker is described in Fig.~\ref{fig:SupportStructureparametrization}, which shows the parametrization used for the support cone structure of the inner tracker. 
Some parameters have been considered fixed and other free to vary within their ranges.
Parameters that are fixed typically do not have much room for optimization considering the constraints of the design and potential overlaps. 
The non-projective design can be realised by fixing the support structure angle to ($\theta = 36.5\degree$) shown in \ref{fig:SupportStructureparametrization}. Therefore, the non-projective design solutions are a subset of solutions that can be achieved by this parameterization.  

\begin{figure}[h!]
    \centering
    \includegraphics[width=0.45\textwidth]{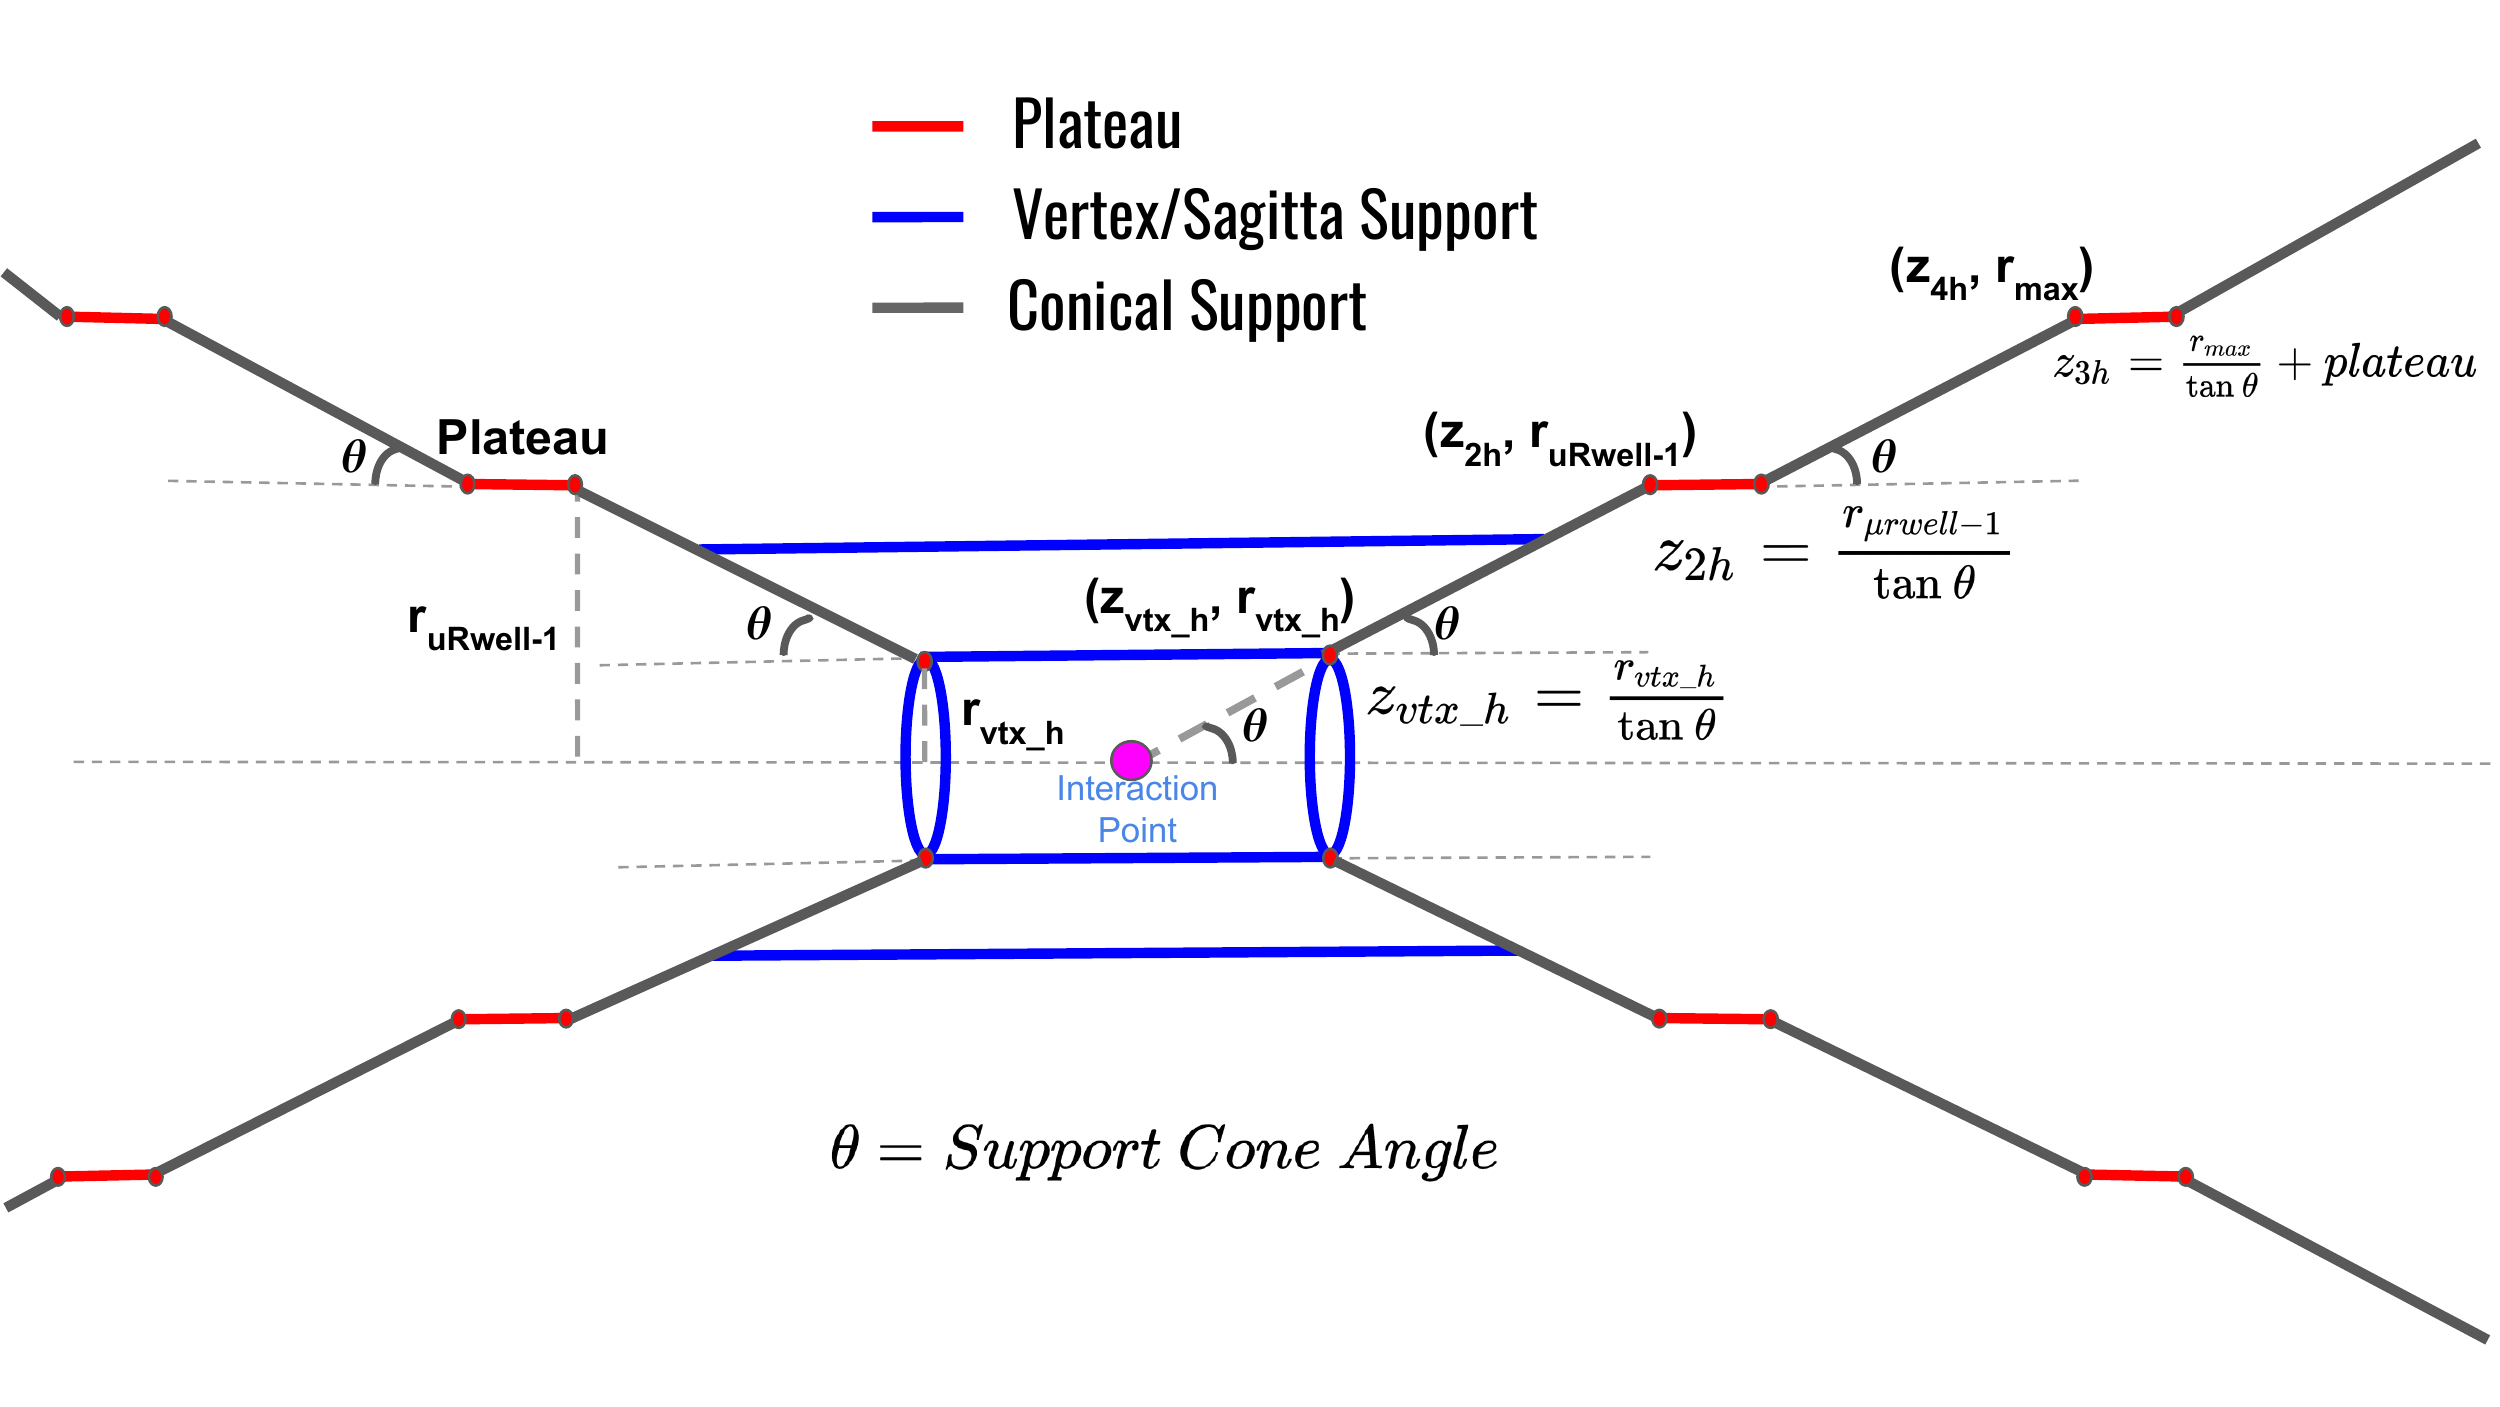}
    \caption{\textbf{Parametrization of the support cone for the inner tracker:} The inner tracker support is characterised by five variables: $\theta$ (the angle of projection of the support cone structure), $r_{vtx}$ (radius of vertex support structure), $r_{\mu rwell-1}$ $\mu$Rwell-1 radius, plateau length, $r_{max}$ maximum allowed radius of inner tracker).
    %\cris{$\mu$RWELL -1: penultimate? Does not appear in figure dubbed this way.}
    %\textbf{It is uRwell-1 is penultimate. }
    }
    \label{fig:SupportStructureparametrization}
\end{figure}
